# Supplementary material for: Semilocal exchange-correlation potentials for solid-state calculations: Current status and future directions
Source: arXiv:1908.01820 ancillary file (2019-09-18)
Supplement: Supplementary file 1 [file Supplementary_material.pdf]

# Supplementary material

## Semilocal exchange-correlation potentials for solid-state calculations: Current status and future directions

Fabien Tran,[1] Jan Doumont,[1] Leila Kalantari,[1] Ahmad W. Huran,[2] Miguel A. L. Marques,[2] and Peter Blaha[1]

[1]*Institute of Materials Chemistry, Vienna University of Technology, Getreidemarkt 9/165-TC, A-1060 Vienna, Austria*

[2]*Institut für Physik, Martin-Luther-Universität Halle-Wittenberg, D-06099 Halle, Germany*

TABLE SI: Calculated (with the WIEN2K code) and experimental band gaps (in eV). The contribution from the exchange derivative discontinuity to the GLLB-SC band gap is indicated in parenthesis. The second and third columns show the identification numbers of the solids in the materials project (MP)[1] and inorganic crystal structure database (ICSD).[2,3] The references for the experimental values can be found in Ref. 4.

| Solid | MP | ICSD | PBE | EV93PW91 | AK13 | GLLB-SC | Expt. |
|---|---|---|---|---|---|---|---|
| $Ag_2CrO_4$ | mp-557056 | 16298 | 1.42 | 1.55 | 1.64 | 2.51 (0.61) | 1.75 |
| $Ag_2GeS_3$ | mp-9900 | 41711 | 0.10 | 0.54 | 0.91 | 0.78 (0.24) | 1.98 |
| $Ag_2MoO_4$ | mp-19318 | 238013 | 2.27 | 2.83 | 3.64 | 4.44 (1.44) | 3.40 |
| $Ag_2O$ | mp-353 | 247821 | 0.07 | 0.13 | 0.49 | 0.32 (0.10) | 1.30 |
| $Ag_2PdO_2$ | mp-5495 | 51498 | 0.04 | 0.24 | 0.61 | 0.55 (0.17) | 0.18 |
| $Ag_2S$ | mp-610517 | 44507 | 0.66 | 0.84 | 1.10 | 1.17 (0.35) | 0.85 |
| $Ag_2Se$ | mp-568936 | 260148 | 0.00 | 0.00 | 0.02 | 0.00 (0.00) | 0.15 |
| $Ag_3AsS_3$ | mp-4431 | 61806 | 1.02 | 1.42 | 1.87 | 2.09 (0.61) | 2.13 |
| $Ag_3SbS_3$ | mp-4515 | 64986 | 0.90 | 1.32 | 1.78 | 2.00 (0.59) | 1.93 |
| $Ag_5IO_6$ | mp-554648 | 415893 | 0.00 | 0.14 | 0.58 | 0.42 (0.14) | 1.40 |
| $AgAlO_2$ | mp-11794 | 99688 | 0.86 | 1.32 | 2.14 | 2.45 (0.85) | 2.95 |
| $AgAlS_2$ | mp-5782 | 604692 | 2.07 | 2.75 | 3.76 | 3.94 (1.23) | 3.13 |
| $AgAlSe_2$ | mp-14091 | 604704 | 1.02 | 1.64 | 2.49 | 2.30 (0.71) | 2.55 |
| $AgAlTe_2$ | mp-14092 | 28746 | 1.16 | 1.66 | 2.32 | 2.27 (0.67) | 2.35 |
| $AgBiP_2S_6$ | mp-556434 | 170639 | 1.17 | 1.46 | 1.81 | 2.53 (0.74) | 1.70 |
| $AgBiP_2Se_6$ | mp-569126 | 195334 | 1.32 | 1.70 | 2.15 | 2.38 (0.70) | 1.40 |
| AgBr | mp-23231 | 65061 | 0.68 | 1.47 | 2.41 | 1.86 (0.60) | 2.71 |
| AgCl | mp-22922 | 64734 | 0.93 | 1.74 | 2.80 | 2.46 (0.81) | 3.25 |
| AgF | mp-7592 | 18008 | 0.00 | 0.22 | 1.34 | 1.02 (0.38) | 2.80 |
| $AgGaS_2$ | mp-5342 | 605187 | 1.21 | 1.84 | 2.48 | 2.53 (0.77) | 2.71 |
| $AgGaSe_2$ | mp-5518 | 52570 | 0.52 | 1.14 | 1.66 | 1.37 (0.42) | 1.81 |
| $AgGaTe_2$ | mp-4899 | 71007 | 0.30 | 0.76 | 1.04 | 0.76 (0.22) | 1.32 |
| AgI | mp-22894 | 56553 | 1.48 | 2.09 | 3.02 | 2.71 (0.86) | 3.02 |
| AgI | mp-22925 | 56552 | 1.34 | 2.02 | 3.01 | 2.55 (0.81) | 2.91 |
| $AgInO_2$ | mp-22660 | 202429 | 0.36 | 0.71 | 1.30 | 1.38 (0.41) | 1.90 |
| $AgInS_2$ | mp-19833 | 51617 | 0.48 | 1.08 | 1.72 | 1.57 (0.49) | 2.04 |
| $AgInSe_2$ | mp-20554 | 52583 | 0.04 | 0.63 | 1.18 | 0.74 (0.23) | 1.24 |
| $AgInTe_2$ | mp-22386 | 236191 | 0.27 | 0.77 | 1.13 | 0.80 (0.24) | 0.96 |
| $AgScP_2Se_6$ | mp-13383 | 195336 | 1.54 | 1.72 | 2.02 | 2.89 (0.82) | 1.55 |
| $Al_2O_3$ | mp-1143 | 31545 | 6.20 | 6.62 | 7.88 | 9.75 (2.57) | 8.80 |
| AlAs | mp-2172 | 656315 | 1.47 | 1.92 | 2.77 | 2.60 (0.86) | 2.23 |
| AlN | mp-661 | 602460 | 4.14 | 4.43 | 5.30 | 6.52 (1.87) | 6.11 |
| AlP | mp-1550 | 52649 | 1.59 | 2.13 | 3.02 | 2.84 (0.94) | 2.45 |
| $AlPO_4$ | mp-3955 | 50100 | 5.96 | 6.56 | 8.71 | 10.08 (2.83) | 7.89 |
| AlSb | mp-2624 | 609288 | 1.22 | 1.58 | 2.29 | 2.00 (0.67) | 1.69 |
| Ar | mp-23155 | 24788 | 8.71 | 9.27 | 15.12 | 15.00 (4.71) | 14.15 |
| $As_2S_3$ | mp-641 | 15239 | 1.86 | 2.20 | 2.65 | 3.19 (0.97) | 2.60 |
| $As_2Se_3$ | mp-909 | 44058 | 1.20 | 1.50 | 1.90 | 2.13 (0.66) | 2.15 |
| $As_2Te_3$ | mp-484 | 196146 | 0.39 | 0.46 | 0.56 | 0.65 (0.21) | 0.90 |
| $AsI_3$ | mp-23218 | 56571 | 2.11 | 2.29 | 2.57 | 3.29 (1.01) | 2.47 |
| B | mp-160 | 431643 | 0.97 | 1.02 | 1.22 | 1.34 (0.37) | 2.00 |
| $B_{12}P_2$ | mp-28395 | 62748 | 2.42 | 2.59 | 2.85 | 3.51 (1.03) | 3.35 |
| $Ba_2BiInS_5$ | mp-864638 | 261678 | 1.23 | 1.65 | 2.08 | 2.35 (0.70) | 1.55 |
| $Ba_2Cu_2ThSe_5$ | mp-1078405 | 195762 | 0.68 | 0.96 | 1.50 | 1.80 (0.55) | 1.75 |
| $Ba_2InTaO_6$ | mp-1079630 | 261480 | 4.20 | 4.42 | 4.72 | 6.95 (1.65) | 4.17 |
| $Ba_3MgTa_2O_9$ | mp-6325 | 240279 | 3.41 | 3.67 | 4.02 | 5.97 (1.45) | 4.28 |
| $Ba_3ThSe_7$ | mp-1095255 | 429804 | 0.91 | 1.18 | 1.54 | 1.91 (0.62) | 1.96 |
| $BaAg_2GeS_4$ | mp-7394 | 10040 | 0.58 | 1.19 | 1.83 | 1.50 (0.45) | 2.02 |
| $BaAg_2SnS_4$ | mp-555166 | 41898 | 0.42 | 0.93 | 1.50 | 1.31 (0.39) | 1.77 |
| $BaBiBS_4$ | mp-861618 | 248222 | 1.99 | 2.31 | 2.63 | 3.51 (1.05) | 2.34 |
| $BaBiO_2Cl$ | mp-552806 | 79532 | 3.31 | 3.71 | 4.37 | 5.59 (1.55) | 3.71 |
| $BaCl_2$ | mp-23199 | 262674 | 5.04 | 5.64 | 6.95 | 8.77 (2.53) | 7.00 |
| $BaCu_2GeS_4$ | mp-17947 | 10006 | 1.23 | 1.53 | 1.77 | 2.63 (0.81) | 2.47 |
| $BaCu_2S_2$ | mp-5970 | 89573 | 0.91 | 1.23 | 1.67 | 2.29 (0.70) | 2.10 |
| $BaCu_2SnSe_4$ | mp-12364 | 170857 | 0.58 | 1.67 | 1.07 | 1.80 (0.56) | 1.72 |

TABLE SI: (*Continued.*)

| Solid | MP | ICSD | PBE | EV93PW91 | AK13 | GLLB-SC | Expt. |
|---|---|---|---|---|---|---|---|
| BaCuTeF | mp-13287 | 245624 | 1.00 | 1.21 | 1.57 | 1.83 (0.58) | 2.30 |
| $BaF_2$ | mp-1029 | 64717 | 6.86 | 7.47 | 9.63 | 12.65 (3.65) | 9.10 |
| $BaGe_2$ | mp-2139 | 409260 | 0.58 | 0.75 | 1.12 | 1.22 (0.42) | 0.97 |
| $BaHgS_2$ | mp-28007 | 251739 | 1.26 | 1.58 | 1.86 | 2.18 (0.70) | 1.93 |
| BaO | mp-1342 | 616005 | 2.08 | 2.52 | 3.56 | 4.70 (1.32) | 4.80 |
| BaS | mp-1500 | 52690 | 2.22 | 2.80 | 4.03 | 4.59 (1.54) | 3.81 |
| $BaSbBS_4$ | mp-866301 | 248221 | 2.46 | 2.73 | 3.09 | 4.15 (1.27) | 2.70 |
| BaSe | mp-1253 | 52696 | 1.99 | 2.50 | 3.67 | 4.08 (1.39) | 3.42 |
| $BaSi_2$ | mp-1477 | 185375 | 0.79 | 1.01 | 1.44 | 1.59 (0.55) | 1.15 |
| $BaSnO_3$ | mp-3163 | 239582 | 0.97 | 1.33 | 1.74 | 3.12 (0.83) | 3.70 |
| BaTe | mp-1000 | 616165 | 1.60 | 2.09 | 3.23 | 3.23 (1.14) | 3.40 |
| $BaTeMo_2O_9$ | mp-19049 | 281503 | 2.91 | 2.96 | 3.09 | 4.60 (1.10) | 2.95 |
| $BaZn_2As_2$ | mp-570198 | 417000 | 0.00 | 0.00 | 0.48 | 0.00 (0.00) | 0.23 |
| BaZnOS | mp-548469 | 171239 | 2.32 | 2.78 | 3.57 | 4.25 (1.23) | 3.90 |
| BeO | mp-2542 | 391224 | 7.37 | 7.94 | 9.15 | 10.99 (2.85) | 10.59 |
| BeSe | mp-1541 | 616419 | 2.66 | 3.19 | 4.25 | 4.26 (1.30) | 5.50 |
| BeTe | mp-252 | 616439 | 2.00 | 2.43 | 3.23 | 3.07 (0.96) | 2.80 |
| $Bi_2O_2CO_3$ | mp-30200 | 252588 | 0.00 | 0.00 | 0.11 | 0.81 (0.20) | 3.42 |
| $Bi_2O_3$ | mp-23262 | 94229 | 2.40 | 2.69 | 3.17 | 4.17 (1.14) | 2.50 |
| $Bi_2O_3$ | mp-23195 | 189995 | 1.59 | 1.83 | 2.25 | 3.30 (0.99) | 2.28 |
| $Bi_2S_3$ | mp-22856 | 153946 | 1.38 | 1.74 | 2.22 | 2.62 (0.80) | 1.45 |
| $Bi_2Se_3$ | mp-541837 | 165226 | 0.18 | 0.56 | 1.04 | 0.70 (0.21) | 0.22 |
| $Bi_2Te_3$ | mp-34202 | 193330 | 0.27 | 0.53 | 0.61 | 0.62 (0.19) | 0.15 |
| BiCuOSe | mp-23116 | 189174 | 0.29 | 0.57 | 0.85 | 1.58 (0.43) | 0.82 |
| $BiF_3$ | mp-557466 | 25567 | 3.77 | 4.08 | 4.45 | 7.43 (1.89) | 3.94 |
| $BiI_3$ | mp-22849 | 53634 | 2.40 | 2.71 | 2.99 | 3.92 (1.20) | 1.67 |
| $BiNSr_3$ | mp-570008 | 152053 | 0.26 | 0.33 | 1.10 | 1.52 (0.52) | 0.89 |
| BiOBr | mp-23072 | 61225 | 2.15 | 2.52 | 3.10 | 3.96 (1.14) | 2.92 |
| BiOCl | mp-22939 | 195115 | 2.65 | 3.02 | 3.62 | 4.62 (1.30) | 3.46 |
| BiOI | mp-22987 | 391354 | 1.58 | 1.99 | 2.50 | 3.06 (0.90) | 1.89 |
| BiSBr | mp-23324 | 31389 | 1.98 | 2.39 | 2.85 | 3.44 (1.02) | 1.95 |
| BiSCl | mp-23318 | 100173 | 1.85 | 2.24 | 2.75 | 3.23 (0.94) | 1.89 |
| BiSeBr | mp-569707 | 76649 | 1.01 | 1.26 | 1.53 | 2.04 (0.63) | 1.50 |
| BiSeI | mp-23020 | 280311 | 1.48 | 1.86 | 2.22 | 2.80 (0.84) | 1.30 |
| BiSI | mp-23514 | 23631 | 1.75 | 2.15 | 2.54 | 3.21 (0.97) | 1.56 |
| BN | mp-1639 | 77271 | 4.46 | 4.84 | 5.70 | 6.69 (1.67) | 6.36 |
| BN | mp-984 | 241875 | 4.26 | 4.64 | 5.44 | 7.29 (2.00) | 5.96 |
| BP | mp-1479 | 602964 | 1.25 | 1.48 | 2.02 | 1.87 (0.54) | 2.10 |
| C | mp-66 | 190650 | 4.14 | 4.30 | 4.78 | 5.45 (1.29) | 5.50 |
| $Ca_2Pb$ | mp-30478 | 58920 | 0.15 | 0.14 | 0.71 | 0.53 (0.19) | 0.46 |
| $Ca_2Si$ | mp-2517 | 158275 | 0.35 | 0.48 | 1.14 | 1.10 (0.40) | 1.90 |
| $Ca_2Sn$ | mp-22735 | 659611 | 0.15 | 0.18 | 0.79 | 0.67 (0.24) | 0.90 |
| $Ca_2SnS_4$ | mp-866503 | 429695 | 2.45 | 2.90 | 3.42 | 4.43 (1.36) | 2.32 |
| $CaB_6$ | mp-865 | 196516 | 0.03 | 0.14 | 0.64 | 0.28 (0.09) | 1.15 |
| $CaCl_2$ | mp-23214 | 246416 | 5.42 | 5.92 | 6.98 | 9.87 (3.06) | 6.90 |
| $CaCO_3$ | mp-3953 | 52151 | 5.18 | 5.50 | 5.89 | 8.86 (2.25) | 6.00 |
| $CaF_2$ | mp-2741 | 82707 | 7.28 | 8.10 | 9.85 | 12.96 (3.63) | 12.10 |
| $CaH_2$ | mp-23713 | 260873 | 2.97 | 3.57 | 5.02 | 5.82 (1.72) | 4.40 |
| $CaMg_2N_2$ | mp-5795 | 79123 | 2.10 | 2.28 | 3.27 | 4.15 (1.36) | 3.25 |
| CaO | mp-2605 | 261847 | 3.67 | 4.09 | 5.04 | 7.33 (1.95) | 6.88 |
| CaS | mp-1672 | 603165 | 2.39 | 2.93 | 3.99 | 4.72 (1.45) | 4.43 |
| CaSe | mp-1415 | 52788 | 2.06 | 2.51 | 3.52 | 4.13 (1.29) | 3.85 |
| $CaSnO_3$ | mp-4438 | 193658 | 2.70 | 3.02 | 3.45 | 5.00 (1.41) | 4.40 |
| CaZnOS | mp-7204 | 245309 | 2.76 | 3.45 | 4.43 | 4.83 (1.42) | 3.70 |
| $CdAl_2S_4$ | mp-5928 | 83526 | 2.88 | 3.52 | 4.31 | 4.94 (1.50) | 3.58 |
| $CdAs_2$ | mp-471 | 609931 | 0.29 | 0.62 | 0.88 | 0.58 (0.18) | 0.99 |
| $CdGa_2S_4$ | mp-4452 | 31354 | 2.04 | 2.63 | 3.24 | 3.55 (1.06) | 3.31 |
| $CdGa_2Se_4$ | mp-3772 | 30908 | 1.51 | 2.14 | 2.76 | 2.64 (0.80) | 2.16 |
| $CdGa_2Te_4$ | mp-13949 | 25646 | 1.36 | 1.86 | 2.30 | 2.20 (0.65) | 1.45 |
| $CdGeAs_2$ | mp-4953 | 42098 | 0.10 | 0.31 | 0.56 | 0.04 (0.01) | 0.67 |
| $CdGeP_2$ | mp-3668 | 100467 | 0.91 | 1.41 | 1.75 | 1.75 (0.50) | 1.73 |

TABLE SI: (*Continued.*)

| Solid | MP | ICSD | PBE | EV93PW91 | AK13 | GLLB-SC | Expt. |
|---|---|---|---|---|---|---|---|
| $CdI_2$ | mp-567259 | 43852 | 2.35 | 2.77 | 3.22 | 3.68 (1.15) | 3.47 |
| $CdIn_2S_4$ | mp-559200 | 252372 | 1.15 | 1.78 | 2.36 | 2.41 (0.71) | 2.44 |
| $CdIn_2Se_4$ | mp-568032 | 151953 | 0.98 | 1.55 | 2.15 | 1.98 (0.62) | 1.55 |
| $CdIn_2Se_4$ | mp-22304 | 151954 | 0.96 | 1.56 | 2.19 | 1.91 (0.60) | 1.46 |
| $CdP_4$ | mp-7904 | 25605 | 0.32 | 0.64 | 1.20 | 0.81 (0.25) | 1.15 |
| CdS | mp-672 | 154186 | 1.22 | 1.95 | 2.88 | 2.50 (0.77) | 2.48 |
| CdSb | mp-1321 | 52830 | 0.14 | 0.41 | 0.68 | 0.31 (0.09) | 0.46 |
| $CdSb_2Se_3Br_2$ | mp-567556 | 159464 | 1.06 | 1.33 | 1.68 | 1.98 (0.60) | 1.40 |
| CdSe | mp-2691 | 187310 | 0.71 | 1.45 | 2.23 | 1.62 (0.50) | 1.74 |
| CdSe | mp-1070 | 415785 | 0.73 | 1.45 | 2.23 | 1.65 (0.51) | 1.73 |
| $CdSiAs_2$ | mp-3078 | 22187 | 0.81 | 1.31 | 1.71 | 1.62 (0.47) | 1.55 |
| $CdSiP_2$ | mp-4666 | 23696 | 1.35 | 1.77 | 2.49 | 2.35 (0.75) | 2.08 |
| $CdSnAs_2$ | mp-3829 | 44258 | 0.09 | 0.22 | 0.54 | 0.09 (0.03) | 0.26 |
| $CdSnO_3$ | mp-754329 | 181930 | 1.11 | 1.57 | 2.24 | 2.81 (0.86) | 3.10 |
| $CdSnP_2$ | mp-5213 | 44257 | 0.54 | 1.10 | 1.51 | 1.31 (0.39) | 1.23 |
| CdTe | mp-406 | 161693 | 0.77 | 1.40 | 1.98 | 1.47 (0.44) | 1.48 |
| $CrSi_2$ | mp-1222 | 161434 | 0.37 | 0.41 | 0.56 | 0.86 (0.23) | 0.35 |
| $Cs_2AgBiBr_6$ | mp-1078250 | 291597 | 1.28 | 1.77 | 2.13 | 2.63 (0.77) | 2.19 |
| $Cs_2AgBiCl_6$ | mp-1078258 | 291598 | 1.87 | 2.31 | 2.74 | 3.43 (0.97) | 2.77 |
| $Cs_2AgVS_4$ | mp-8684 | 50460 | 1.41 | 1.51 | 1.68 | 2.32 (0.56) | 1.77 |
| $Cs_2Au_2Br_6$ | mp-569548 | 170696 | 0.89 | 0.91 | 0.95 | 1.59 (0.48) | 1.60 |
| $Cs_2Au_2Cl_6$ | mp-23484 | 6061 | 1.08 | 1.04 | 1.08 | 1.98 (0.58) | 2.04 |
| $Cs_2Au_2I_6$ | mp-28453 | 59269 | 0.84 | 0.87 | 0.90 | 1.46 (0.47) | 1.31 |
| $Cs_2Cd_3Te_4$ | mp-567386 | 90369 | 1.76 | 2.29 | 2.61 | 3.10 (0.97) | 2.48 |
| $Cs_2Hg_3I_8$ | mp-540574 | 4074 | 1.86 | 2.26 | 2.68 | 3.02 (0.96) | 2.56 |
| $Cs_2SnBr_6$ | mp-641923 | 158957 | 1.19 | 1.60 | 2.16 | 2.68 (0.88) | 2.70 |
| $Cs_2SnCl_6$ | mp-608555 | 9023 | 2.92 | 3.32 | 4.00 | 5.37 (1.62) | 3.90 |
| $Cs_2TeBr_6$ | mp-23405 | 65058 | 1.97 | 2.18 | 2.55 | 3.31 (0.99) | 2.20 |
| $Cs_2TeI_6$ | mp-540957 | 38105 | 1.38 | 1.61 | 1.90 | 2.43 (0.79) | 1.52 |
| $Cs_2TiAg_2S_4$ | mp-10488 | 280645 | 1.57 | 1.81 | 2.02 | 2.84 (0.77) | 2.44 |
| $Cs_3Bi_2Br_9$ | mp-27544 | 1142 | 2.53 | 2.82 | 3.27 | 4.18 (1.21) | 2.50 |
| $Cs_3Bi_2I_9$ | mp-624214 | 23124 | 2.09 | 2.37 | 2.82 | 3.43 (1.05) | 1.80 |
| $Cs_3Sb$ | mp-10378 | 53243 | 0.81 | 1.42 | 2.26 | 2.61 (0.88) | 1.60 |
| $Cs_3Sb_2Br_9$ | mp-579560 | 39824 | 1.61 | 1.79 | 2.03 | 2.74 (0.81) | 2.30 |
| $Cs_3Sb_2I_9$ | mp-23029 | 84989 | 1.63 | 1.83 | 2.24 | 2.62 (0.81) | 1.89 |
| CsAu | mp-2667 | 58427 | 1.01 | 1.41 | 2.79 | 3.11 (1.03) | 2.50 |
| $CsLaHgSe_3$ | mp-11124 | 281441 | 1.53 | 2.02 | 2.55 | 2.69 (0.87) | 2.46 |
| $CsPbBr_3$ | mp-567629 | 97851 | 1.81 | 2.21 | 2.79 | 3.21 (0.89) | 2.32 |
| $CsSnBr_3$ | mp-27214 | 4071 | 0.38 | 0.60 | 1.06 | 0.96 (0.27) | 1.75 |
| $CsSnCl_3$ | mp-27394 | 14199 | 2.91 | 3.27 | 3.99 | 4.25 (1.02) | 2.80 |
| $CsSnI_3$ | mp-568570 | 69996 | 0.52 | 0.63 | 0.95 | 1.00 (0.30) | 1.31 |
| $CsYCdSe_3$ | mp-11116 | 281433 | 2.21 | 2.67 | 3.34 | 3.89 (1.17) | 2.48 |
| $CsYHgSe_3$ | mp-11123 | 281440 | 1.51 | 2.01 | 2.52 | 2.65 (0.82) | 2.54 |
| $CsYZnSe_3$ | mp-574620 | 280847 | 2.17 | 2.58 | 3.24 | 3.85 (1.16) | 2.29 |
| $Cu_2CdGeS_4$ | mp-13982 | 26150 | 0.63 | 1.03 | 1.42 | 1.95 (0.57) | 2.05 |
| $Cu_2CdGeSe_4$ | mp-10967 | 95235 | 0.00 | 0.33 | 0.64 | 0.68 (0.21) | 1.20 |
| $Cu_2GeS_3$ | mp-15252 | 85138 | 0.29 | 0.53 | 0.69 | 1.24 (0.36) | 1.53 |
| $Cu_2GeSe_3$ | mp-4728 | 160386 | 0.00 | 0.00 | 0.00 | 0.00 (0.00) | 0.82 |
| $Cu_2GeSe_3$ | mp-677105 | 192171 | 0.00 | 0.11 | 0.17 | 0.25 (0.08) | 0.78 |
| $Cu_2O$ | mp-361 | 172174 | 0.59 | 0.55 | 0.72 | 1.00 (0.30) | 2.17 |
| $Cu_2S$ | mp-618991 | 16550 | 0.09 | 0.31 | 0.64 | 0.78 (0.24) | 1.04 |
| $Cu_2Se$ | mp-16366 | 56025 | 0.00 | 0.00 | 0.00 | 0.00 (0.00) | 1.20 |
| $Cu_2S$ | mp-553942 | 20560 | 0.00 | 0.00 | 0.02 | 0.00 (0.00) | 1.21 |
| $Cu_2SnS_3$ | mp-10519 | 91762 | 0.10 | 0.21 | 0.38 | 0.68 (0.20) | 0.86 |
| $Cu_2SnSe_3$ | mp-11658 | 97966 | 0.05 | 0.06 | 0.08 | 0.09 (0.03) | 0.84 |
| $Cu_2Te$ | mp-1861 | 77055 | 0.00 | 0.00 | 0.00 | 0.00 (0.00) | 0.90 |
| $Cu_2ZnGeSe_4$ | mp-10824 | 93409 | 0.00 | 0.26 | 0.53 | 0.60 (0.18) | 1.29 |
| $Cu_2ZnSiS_4$ | mp-977414 | 261367 | 1.27 | 1.61 | 2.08 | 2.93 (0.84) | 2.97 |
| $Cu_2ZnSnS_4$ | mp-1025500 | 184478 | 0.46 | 0.86 | 1.26 | 1.76 (0.52) | 1.51 |
| $Cu_3AsS_4$ | mp-3345 | 413350 | 0.22 | 0.43 | 0.56 | 1.10 (0.32) | 1.24 |
| $Cu_3AsSe_4$ | mp-675626 | 610361 | 0.00 | 0.00 | 0.00 | 0.00 (0.00) | 0.88 |

TABLE SI: (*Continued.*)

| Solid | MP | ICSD | PBE | EV93PW91 | AK13 | GLLB-SC | Expt. |
|---|---|---|---|---|---|---|---|
| $Cu_3PS_4$ | mp-3934 | 412240 | 1.24 | 1.49 | 1.73 | 2.70 (0.78) | 2.35 |
| $Cu_3PSe_4$ | mp-5756 | 95412 | 0.26 | 0.55 | 0.77 | 1.11 (0.33) | 1.40 |
| $Cu_3SbS_4$ | mp-5702 | 412239 | 0.00 | 0.07 | 0.24 | 0.56 (0.17) | 0.88 |
| $Cu_3SbSe_4$ | mp-9814 | 400652 | 0.00 | 0.00 | 0.00 | 0.00 (0.00) | 0.29 |
| $CuAlO_2$ | mp-3748 | 60844 | 1.92 | 2.00 | 2.35 | 3.39 (0.96) | 2.99 |
| $CuAlS_2$ | mp-4979 | 42124 | 1.88 | 2.33 | 3.04 | 4.07 (1.22) | 3.45 |
| $CuAlSe_2$ | mp-8016 | 28734 | 1.12 | 1.61 | 2.30 | 2.78 (0.84) | 2.68 |
| $CuBiP_2Se_6$ | mp-569715 | 195341 | 0.78 | 1.05 | 1.36 | 2.20 (0.64) | 1.20 |
| CuBr | mp-22913 | 78274 | 0.46 | 1.01 | 1.86 | 2.19 (0.73) | 3.07 |
| $CuBS_2$ | mp-12954 | 156413 | 1.67 | 1.91 | 2.42 | 3.11 (0.91) | 3.61 |
| CuCl | mp-22914 | 78270 | 0.54 | 1.07 | 2.01 | 2.57 (0.85) | 3.40 |
| $CuGaO_2$ | mp-4280 | 60846 | 0.93 | 1.06 | 1.45 | 2.12 (0.61) | 2.55 |
| $CuGaS_2$ | mp-5238 | 66864 | 0.87 | 1.27 | 1.66 | 2.29 (0.67) | 2.51 |
| $CuGaSe_2$ | mp-4840 | 42097 | 0.18 | 0.61 | 0.94 | 1.05 (0.31) | 1.70 |
| $CuGaTe_2$ | mp-3839 | 74456 | 0.58 | 0.97 | 1.18 | 1.33 (0.39) | 1.23 |
| CuI | mp-22895 | 33724 | 1.16 | 1.71 | 2.40 | 2.65 (0.82) | 3.12 |
| $CuInS_2$ | mp-22736 | 186714 | 0.29 | 0.71 | 1.17 | 1.64 (0.50) | 1.53 |
| $CuInSe_2$ | mp-22811 | 252780 | 0.03 | 0.24 | 0.63 | 0.64 (0.20) | 1.04 |
| $CuInTe_2$ | mp-22261 | 74460 | 0.11 | 0.50 | 0.76 | 0.68 (0.20) | 1.06 |
| $CuLaO_2$ | mp-20072 | 18102 | 2.57 | 2.78 | 3.44 | 4.92 (1.50) | 2.34 |
| $CuSbSe_2$ | mp-20331 | 418754 | 0.58 | 0.73 | 0.96 | 1.52 (0.46) | 1.04 |
| $CuScO_2$ | mp-4636 | 55689 | 2.38 | 2.50 | 2.81 | 4.23 (1.26) | 3.30 |
| $CuTaN_2$ | mp-8927 | 71136 | 0.92 | 1.10 | 1.43 | 2.19 (0.66) | 1.50 |
| $FeP_2$ | mp-20027 | 15027 | 0.38 | 0.45 | 0.65 | 0.89 (0.26) | 0.37 |
| $FeS_2$ | mp-226 | 109377 | 0.66 | 0.68 | 0.82 | 1.73 (0.52) | 0.95 |
| $Ga_2S_3$ | mp-539 | 409550 | 1.89 | 2.46 | 3.07 | 3.51 (0.98) | 3.44 |
| GaAs | mp-2534 | 107946 | 0.52 | 1.12 | 1.44 | 1.04 (0.29) | 1.52 |
| GaN | mp-804 | 157398 | 1.86 | 2.19 | 2.63 | 3.15 (0.91) | 3.50 |
| GaP | mp-2490 | 77087 | 1.59 | 2.09 | 2.62 | 2.56 (0.77) | 2.35 |
| GaS | mp-2507 | 173940 | 1.55 | 2.02 | 2.77 | 2.70 (0.80) | 2.54 |
| GaSb | mp-1156 | 635318 | 0.12 | 0.60 | 0.77 | 0.33 (0.09) | 0.82 |
| GaSe | mp-1943 | 63122 | 0.93 | 1.51 | 2.07 | 1.74 (0.48) | 2.10 |
| GaTe | mp-542812 | 8249 | 0.99 | 1.31 | 1.62 | 1.58 (0.47) | 1.80 |
| Ge | mp-32 | 184252 | 0.06 | 0.58 | 0.71 | 0.25 (0.07) | 0.74 |
| GeAs | mp-9548 | 86361 | 0.33 | 0.71 | 1.06 | 0.62 (0.11) | 0.65 |
| $GeAs_2$ | mp-17524 | 23872 | 0.59 | 0.92 | 1.34 | 1.11 (0.33) | 1.06 |
| $GeO_2$ | mp-470 | 92551 | 1.84 | 2.18 | 2.66 | 3.91 (0.97) | 5.35 |
| GeSe | mp-700 | 41738 | 0.68 | 0.85 | 1.19 | 1.33 (0.42) | 1.07 |
| HfNBr | mp-568346 | 95720 | 2.07 | 2.29 | 2.58 | 3.81 (0.91) | 3.10 |
| $HfO_2$ | mp-352 | 173158 | 4.04 | 4.43 | 4.97 | 7.07 (1.67) | 5.50 |
| $HfS_2$ | mp-985829 | 601164 | 0.92 | 1.26 | 1.74 | 1.99 (0.57) | 1.96 |
| $HfSe_2$ | mp-985831 | 195308 | 0.42 | 0.67 | 1.13 | 1.17 (0.34) | 1.13 |
| $Hg_2I_2$ | mp-22859 | 262368 | 1.66 | 1.94 | 2.15 | 2.58 (0.80) | 3.00 |
| $Hg_4As_2CdI_4$ | mp-570838 | 416973 | 0.79 | 1.24 | 1.53 | 1.50 (0.46) | 1.45 |
| $HgGa_2S_4$ | mp-4809 | 67220 | 1.74 | 2.29 | 2.83 | 2.94 (0.90) | 2.79 |
| $HgGa_2Se_4$ | mp-4730 | 83712 | 1.10 | 1.65 | 2.14 | 1.93 (0.59) | 1.99 |
| $HgI_2$ | mp-23192 | 181575 | 1.17 | 1.61 | 2.09 | 2.02 (0.65) | 2.40 |
| $HgIn_2Se_4$ | mp-20731 | 25649 | 0.65 | 1.22 | 1.79 | 1.40 (0.44) | 1.16 |
| $HgIn_2Te_4$ | mp-19765 | 25652 | 0.76 | 1.25 | 1.67 | 1.33 (0.40) | 0.90 |
| HgO | mp-1224 | 14124 | 1.22 | 1.38 | 1.69 | 2.28 (0.67) | 1.90 |
| HgS | mp-634 | 81923 | 1.47 | 1.91 | 2.42 | 2.59 (0.74) | 2.03 |
| HgS | mp-1123 | 81917 | 0.00 | 0.10 | 0.62 | 0.00 (0.00) | 0.54 |
| $HgSnO_3$ | mp-13554 | 260029 | 0.00 | 0.33 | 0.81 | 1.10 (0.34) | 1.60 |
| $In_2Se_3$ | mp-19907 | 5419 | 0.00 | 0.00 | 0.00 | 0.00 (0.00) | 1.36 |
| $In_2Se_3$ | mp-20830 | 640498 | 0.00 | 0.00 | 0.00 | 0.00 (0.00) | 1.31 |
| $In_6S_7$ | mp-555853 | 15317 | 0.33 | 0.59 | 0.97 | 0.63 (0.12) | 0.93 |
| $In_6Se_7$ | mp-567596 | 9135 | 0.06 | 0.28 | 0.64 | 0.24 (0.05) | 2.20 |
| InAs | mp-20305 | 41444 | 0.00 | 0.35 | 0.72 | 0.07 (0.02) | 0.42 |
| $InBi_2S_4Cl$ | mp-559521 | 484 | 1.62 | 2.00 | 2.43 | 2.88 (0.87) | 1.50 |
| $InBi_2Se_4Br$ | mp-571169 | 159465 | 1.23 | 1.57 | 1.93 | 2.24 (0.67) | 1.21 |
| InN | mp-22205 | 109463 | 0.00 | 0.13 | 0.52 | 0.31 (0.10) | 0.69 |

TABLE SI: (*Continued.*)

| Solid | MP | ICSD | PBE | EV93PW91 | AK13 | GLLB-SC | Expt. |
|---|---|---|---|---|---|---|---|
| InP | mp-20351 | 41443 | 0.68 | 1.29 | 1.79 | 1.51 (0.44) | 1.42 |
| $InPS_4$ | mp-20790 | 1699 | 2.44 | 2.93 | 3.30 | 4.15 (1.21) | 3.12 |
| InS | mp-19795 | 81338 | 1.17 | 1.53 | 1.89 | 2.01 (0.59) | 2.09 |
| InSb | mp-20012 | 162196 | 0.00 | 0.30 | 0.51 | 0.00 (0.00) | 0.24 |
| $InSb_2S_4Br$ | mp-559864 | 159467 | 1.49 | 1.79 | 2.19 | 2.64 (0.78) | 1.50 |
| $InSb_2S_4Cl$ | mp-556541 | 159468 | 1.53 | 1.82 | 2.21 | 2.66 (0.79) | 1.80 |
| $InSb_2Se_4Br$ | mp-570321 | 159466 | 1.05 | 1.30 | 1.63 | 1.88 (0.57) | 1.21 |
| InTe | mp-20320 | 169418 | 0.00 | 0.00 | 0.28 | 0.00 (0.00) | 1.16 |
| $K_2AgVS_4$ | mp-8900 | 66840 | 1.31 | 1.47 | 1.70 | 2.27 (0.59) | 1.85 |
| $K_2Au_2SnS_4$ | mp-557121 | 74022 | 1.80 | 2.24 | 2.79 | 3.53 (1.04) | 2.75 |
| $K_2AuPS_4$ | mp-9509 | 85679 | 1.40 | 1.85 | 2.62 | 2.99 (0.93) | 2.63 |
| $K_2CsSb$ | mp-581024 | 53237 | 1.06 | 1.64 | 3.07 | 3.05 (1.07) | 1.00 |
| $K_2Hg_3Ge_2S_8$ | mp-11131 | 281506 | 1.57 | 1.96 | 2.43 | 2.71 (0.80) | 2.70 |
| $K_2La_2Ti_3O_{10}$ | mp-6548 | 74193 | 2.16 | 2.38 | 2.64 | 3.94 (0.82) | 3.05 |
| $K_2PbGe_2S_6$ | mp-561132 | 170601 | 2.24 | 2.55 | 2.98 | 3.81 (1.14) | 2.85 |
| $K_2TeBr_6$ | mp-22963 | 22078 | 2.19 | 2.34 | 2.67 | 3.52 (1.03) | 2.17 |
| $K_2TeI_6$ | mp-27688 | 23649 | 1.70 | 1.83 | 2.05 | 2.76 (0.87) | 1.38 |
| $K_2ZnTe_2$ | mp-12535 | 420088 | 2.11 | 2.43 | 3.09 | 3.59 (1.23) | 3.00 |
| $K_3Sb$ | mp-10159 | 44677 | 0.76 | 1.23 | 3.76 | 2.76 (1.06) | 1.40 |
| $K_3Sb$ | mp-14017 | 656327 | 0.47 | 0.86 | 3.74 | 2.37 (1.00) | 1.10 |
| $K_6CdTe_4$ | mp-17698 | 420087 | 1.67 | 2.09 | 3.57 | 3.77 (1.34) | 2.51 |
| $KAg_2PS_4$ | mp-12532 | 420033 | 1.11 | 1.69 | 2.36 | 2.23 (0.66) | 3.02 |
| $KAg_2SbS_4$ | mp-9490 | 82143 | 0.30 | 0.76 | 1.19 | 1.19 (0.36) | 1.71 |
| $KBiSiS_4$ | mp-866651 | 421485 | 2.13 | 2.49 | 2.93 | 3.72 (1.12) | 2.25 |
| KBr | mp-23251 | 187220 | 4.34 | 5.14 | 8.96 | 8.46 (2.85) | 7.80 |
| KCl | mp-23193 | 165593 | 5.21 | 6.04 | 9.79 | 9.89 (3.18) | 8.69 |
| $KCu_3S_2$ | mp-9868 | 100001 | 0.43 | 0.78 | 1.42 | 1.66 (0.51) | 1.64 |
| $KCu_4AsS_4$ | mp-557728 | 420017 | 1.44 | 1.57 | 1.85 | 2.97 (0.90) | 1.90 |
| $KCuThS_3$ | mp-12365 | 170864 | 2.05 | 2.30 | 2.60 | 3.94 (1.19) | 2.95 |
| Kr | mp-612118 | 43726 | 7.26 | 7.96 | 12.81 | 12.39 (4.02) | 11.59 |
| $KTaO_3$ | mp-3614 | 280424 | 2.22 | 2.50 | 2.85 | 4.56 (1.06) | 3.64 |
| $La_2O_3$ | mp-1968 | 56771 | 3.87 | 4.10 | 4.55 | 6.98 (1.90) | 5.34 |
| LaCuOS | mp-6088 | 96343 | 1.68 | 1.86 | 2.17 | 3.39 (0.96) | 3.10 |
| LaCuOSe | mp-552488 | 96758 | 1.54 | 1.71 | 2.02 | 3.15 (0.90) | 2.80 |
| LaCuOTe | mp-546790 | 416522 | 1.19 | 1.33 | 1.66 | 2.29 (0.67) | 2.31 |
| $LaF_3$ | mp-905 | 252346 | 6.38 | 6.30 | 6.31 | 12.36 (2.63) | 10.10 |
| LaZnAsO | mp-549589 | 420204 | 0.52 | 0.78 | 1.09 | 0.99 (0.30) | 1.50 |
| LaZnPO | mp-7060 | 85777 | 0.61 | 0.95 | 1.30 | 1.15 (0.35) | 1.70 |
| $LiAsS_2$ | mp-555874 | 419061 | 1.09 | 1.32 | 1.65 | 1.88 (0.58) | 1.60 |
| $LiAsSe_2$ | mp-1078724 | 248116 | 0.74 | 0.86 | 1.08 | 1.39 (0.44) | 1.11 |
| LiBr | mp-23259 | 52236 | 4.93 | 5.87 | 8.32 | 8.34 (2.57) | 7.60 |
| LiCl | mp-22905 | 26909 | 6.33 | 7.34 | 9.83 | 10.43 (3.10) | 9.40 |
| $LiCoO_2$ | mp-24850 | 51767 | 1.10 | 1.33 | 1.90 | 2.60 (0.67) | 2.10 |
| LiF | mp-1138 | 62361 | 9.08 | 9.87 | 12.56 | 14.95 (4.11) | 13.60 |
| $LiGaTe_2$ | mp-5048 | 162555 | 1.79 | 2.13 | 2.54 | 2.79 (0.88) | 2.65 |
| LiH | mp-23703 | 173177 | 3.08 | 3.75 | 6.21 | 6.49 (2.13) | 4.94 |
| $LiInI_4O_{12}$ | mp-973966 | 422056 | 3.41 | 3.64 | 3.91 | 5.39 (1.48) | 4.27 |
| $LiInSe_2$ | mp-20310 | 60838 | 1.83 | 2.42 | 3.09 | 3.26 (1.02) | 3.01 |
| $LiIO_3$ | mp-22955 | 35473 | 0.58 | 0.66 | 0.79 | 1.56 (0.51) | 6.10 |
| $LiNbO_3$ | mp-3731 | 28294 | 3.46 | 3.57 | 3.74 | 5.96 (1.36) | 3.78 |
| $LiTaO_3$ | mp-3666 | 239372 | 3.30 | 3.53 | 3.74 | 5.85 (1.32) | 4.70 |
| LiZnAs | mp-9124 | 74504 | 0.59 | 1.17 | 1.65 | 1.16 (0.34) | 1.61 |
| LiZnN | mp-7575 | 16790 | 0.66 | 0.81 | 1.17 | 1.59 (0.50) | 1.91 |
| LiZnP | mp-10182 | 642242 | 1.39 | 1.87 | 2.58 | 2.48 (0.78) | 2.04 |
| $Mg_2Ge$ | mp-408 | 81735 | 0.19 | 0.37 | 1.08 | 0.66 (0.24) | 0.69 |
| $Mg_2Si$ | mp-1367 | 180944 | 0.25 | 0.51 | 1.26 | 0.73 (0.27) | 0.78 |
| $Mg_2Sn$ | mp-2343 | 104870 | 0.00 | 0.00 | 0.70 | 0.46 (0.17) | 0.30 |
| $Mg_3Sb_2$ | mp-2646 | 245692 | 0.31 | 0.35 | 1.34 | 1.04 (0.36) | 0.80 |
| $MgCl_2$ | mp-23210 | 86439 | 5.63 | 6.50 | 9.05 | 9.58 (2.80) | 7.50 |
| $MgF_2$ | mp-1249 | 8120 | 7.17 | 8.01 | 11.03 | 12.76 (3.55) | 12.40 |
| MgO | mp-1265 | 9863 | 4.71 | 5.11 | 6.66 | 8.23 (2.33) | 7.67 |

TABLE SI: (*Continued.*)

| Solid | MP | ICSD | PBE | EV93PW91 | AK13 | GLLB-SC | Expt. |
|---|---|---|---|---|---|---|---|
| $MgSiP_2$ | mp-2961 | 22189 | 1.29 | 1.77 | 2.65 | 2.42 (0.82) | 2.41 |
| MgTe | mp-1039 | 642882 | 2.57 | 3.29 | 4.78 | 4.63 (1.47) | 3.49 |
| $MoS_2$ | mp-2815 | 95569 | 0.89 | 1.05 | 1.16 | 1.41 (0.39) | 1.23 |
| $MoSe_2$ | mp-1634 | 601045 | 0.82 | 0.97 | 1.17 | 1.31 (0.38) | 1.09 |
| $MoTe_2$ | mp-602 | 644476 | 0.75 | 0.84 | 0.89 | 1.17 (0.34) | 1.03 |
| $Na_2CdSnS_4$ | mp-561075 | 281233 | 2.00 | 2.59 | 3.50 | 3.96 (1.23) | 1.52 |
| $Na_2KSb$ | mp-15724 | 44332 | 0.76 | 1.19 | 3.38 | 2.43 (0.84) | 1.00 |
| $Na_2TeSe_3$ | mp-573581 | 430312 | 1.26 | 1.57 | 1.94 | 2.34 (0.78) | 1.95 |
| $Na_2Ti_3O_7$ | mp-3488 | 250000 | 3.19 | 3.34 | 3.48 | 5.42 (1.12) | 3.51 |
| $Na_3Sb$ | mp-7956 | 26882 | 0.42 | 0.78 | 2.92 | 1.85 (0.73) | 1.10 |
| $NaAsS_2$ | mp-5942 | 854 | 1.45 | 1.74 | 2.17 | 2.62 (0.84) | 2.23 |
| NaBr | mp-22916 | 41440 | 4.12 | 5.03 | 8.47 | 7.86 (2.57) | 7.10 |
| NaCl | mp-22862 | 181148 | 5.11 | 6.06 | 9.80 | 9.48 (2.99) | 8.75 |
| NaF | mp-682 | 262837 | 6.33 | 7.08 | 11.11 | 12.38 (3.66) | 11.70 |
| NaI | mp-23268 | 61502 | 3.64 | 4.49 | 7.71 | 6.76 (2.21) | 5.80 |
| $NaLa_2TaO_6$ | mp-13019 | 159206 | 4.05 | 4.22 | 4.41 | 7.09 (1.73) | 4.50 |
| $NaSbP_2S_6$ | mp-561303 | 155270 | 2.06 | 2.31 | 2.58 | 3.66 (1.11) | 2.25 |
| $NaTaO_3$ | mp-3858 | 239690 | 2.77 | 3.02 | 3.30 | 5.22 (1.20) | 4.00 |
| $NaYbP_2S_6$ | mp-10838 | 93758 | 0.00 | 0.00 | 0.00 | 0.00 (0.00) | 1.85 |
| Ne | mp-111 | 43427 | 11.59 | 11.55 | 20.66 | 22.09 (6.58) | 21.48 |
| $OsAs_2$ | mp-2455 | 238253 | 0.69 | 0.78 | 0.86 | 1.25 (0.36) | 0.92 |
| $OsP_2$ | mp-2319 | 238252 | 0.78 | 0.82 | 0.91 | 1.45 (0.42) | 1.13 |
| $OsSb_2$ | mp-2695 | 238254 | 0.39 | 0.45 | 0.61 | 0.57 (0.17) | 0.21 |
| P | mp-157 | 417180 | 0.00 | 0.05 | 0.57 | 0.00 (0.00) | 0.31 |
| $P_3N_5$ | mp-567907 | 56876 | 3.67 | 3.92 | 4.40 | 6.33 (1.61) | 5.87 |
| $PbBr_2$ | mp-28077 | 36170 | 3.08 | 3.57 | 4.22 | 5.29 (1.57) | 3.98 |
| $PbCl_2$ | mp-23291 | 27736 | 3.86 | 4.39 | 5.16 | 6.32 (1.81) | 4.86 |
| $PbCrO_4$ | mp-19146 | 40920 | 1.80 | 1.90 | 2.11 | 2.60 (0.60) | 2.25 |
| $PbCuSbS_3$ | mp-649774 | 427413 | 0.64 | 0.89 | 1.25 | 2.02 (0.60) | 1.30 |
| $PbF_2$ | mp-315 | 86738 | 4.42 | 4.84 | 5.76 | 7.42 (1.99) | 5.68 |
| $PbI_2$ | mp-22893 | 68819 | 2.23 | 2.70 | 3.44 | 3.78 (1.15) | 2.28 |
| $PbMoO_4$ | mp-25054 | 239428 | 2.75 | 2.85 | 3.07 | 4.27 (1.00) | 3.60 |
| PbS | mp-21276 | 62190 | 0.32 | 0.80 | 1.56 | 1.03 (0.31) | 0.29 |
| PbSe | mp-2201 | 62195 | 0.26 | 0.66 | 1.32 | 0.87 (0.27) | 0.14 |
| $PbSeO_4$ | mp-22342 | 40921 | 3.62 | 4.05 | 4.70 | 5.33 (0.88) | 4.30 |
| PbTe | mp-19717 | 63098 | 0.80 | 1.09 | 1.44 | 1.48 (0.47) | 0.19 |
| $PbWO_4$ | mp-25176 | 81550 | 3.23 | 3.40 | 3.66 | 4.92 (1.14) | 4.20 |
| PdS | mp-20250 | 61063 | 0.03 | 0.08 | 0.18 | 0.20 (0.06) | 0.50 |
| $PdS_2$ | mp-13682 | 648747 | 0.00 | 0.00 | 0.27 | 0.25 (0.07) | 0.75 |
| $PdSe_2$ | mp-2418 | 170327 | 0.00 | 0.07 | 0.29 | 0.23 (0.06) | 0.40 |
| $PtSb_2$ | mp-562 | 43105 | 0.00 | 0.07 | 0.10 | 0.00 (0.00) | 0.11 |
| $Rb_2AgVS_4$ | mp-8901 | 66841 | 1.37 | 1.51 | 1.71 | 2.33 (0.61) | 1.83 |
| $Rb_2Cu_2SnS_4$ | mp-18006 | 74020 | 1.11 | 1.47 | 1.86 | 3.06 (0.91) | 2.08 |
| $Rb_2CuNbS_4$ | mp-15221 | 84304 | 2.04 | 2.12 | 2.28 | 3.53 (0.99) | 2.64 |
| $Rb_2CuNbSe_4$ | mp-15222 | 84305 | 1.70 | 1.80 | 1.97 | 2.95 (0.85) | 2.19 |
| $Rb_2CuVS_4$ | mp-15219 | 84302 | 1.26 | 1.36 | 1.55 | 2.22 (0.58) | 1.85 |
| $Rb_2TeBr_6$ | mp-23383 | 49521 | 1.90 | 2.12 | 2.48 | 3.19 (0.94) | 2.19 |
| $Rb_2TeI_6$ | mp-28070 | 36009 | 1.48 | 1.67 | 1.92 | 2.51 (0.81) | 1.43 |
| $Rb_2TiCu_2S_4$ | mp-7129 | 280644 | 1.61 | 1.79 | 1.97 | 3.08 (0.85) | 2.19 |
| $Rb_3Sb_2Br_9$ | mp-28222 | 39823 | 1.77 | 1.91 | 2.25 | 2.84 (0.80) | 2.48 |
| $RbAg_2SbS_4$ | mp-17756 | 82145 | 0.82 | 1.25 | 1.63 | 1.68 (0.32) | 2.30 |
| RbAu | mp-30373 | 58428 | 0.34 | 0.74 | 2.31 | 2.18 (0.71) | 2.75 |
| RbBr | mp-22867 | 22167 | 4.34 | 5.13 | 8.77 | 8.47 (2.83) | 7.20 |
| RbCl | mp-23295 | 18016 | 5.06 | 5.85 | 9.47 | 9.76 (3.12) | 8.30 |
| $RbCu_2VS_4$ | mp-15998 | 280516 | 1.11 | 1.19 | 1.33 | 1.91 (0.47) | 1.45 |
| RbF | mp-11718 | 53828 | 5.74 | 6.43 | 10.26 | 11.37 (3.19) | 10.40 |
| RbI | mp-22903 | 22168 | 3.92 | 4.70 | 7.71 | 7.39 (2.53) | 6.37 |
| $ReS_2$ | mp-572758 | 81814 | 1.21 | 1.26 | 1.34 | 1.80 (0.51) | 1.37 |
| $ReSe_2$ | mp-541582 | 81813 | 1.06 | 1.14 | 1.21 | 1.60 (0.45) | 1.19 |
| $RuS_2$ | mp-2030 | 68472 | 0.81 | 0.89 | 1.04 | 1.85 (0.57) | 1.45 |
| $RuSe_2$ | mp-1922 | 68473 | 0.47 | 0.55 | 0.67 | 1.24 (0.39) | 0.76 |

TABLE SI: (*Continued.*)

| Solid | MP | ICSD | PBE | EV93PW91 | AK13 | GLLB-SC | Expt. |
|---|---|---|---|---|---|---|---|
| $RuTe_2$ | mp-1848 | 65169 | 0.10 | 0.22 | 0.36 | 0.60 (0.20) | 0.49 |
| $Sb_2O_3$ | mp-2136 | 240207 | 2.17 | 2.44 | 3.02 | 3.69 (1.09) | 3.25 |
| $Sb_2O_3$ | mp-1999 | 240206 | 3.21 | 3.62 | 4.48 | 5.31 (1.64) | 4.00 |
| $Sb_2S_3$ | mp-2809 | 171850 | 1.29 | 1.53 | 1.91 | 2.23 (0.66) | 1.74 |
| $Sb_2Se_3$ | mp-2160 | 194836 | 0.93 | 1.20 | 1.49 | 1.77 (0.55) | 1.11 |
| $Sb_2Te_3$ | mp-1201 | 193341 | 0.00 | 0.17 | 0.13 | 0.15 (0.04) | 0.28 |
| $SbF_3$ | mp-1880 | 16142 | 4.61 | 4.93 | 5.89 | 7.10 (1.88) | 4.30 |
| $SbI_3$ | mp-569224 | 30906 | 2.31 | 2.57 | 2.91 | 3.76 (1.16) | 2.41 |
| $SbNSr_3$ | mp-7752 | 152052 | 0.26 | 0.35 | 1.14 | 1.57 (0.53) | 1.15 |
| SbSBr | mp-22971 | 88584 | 1.66 | 2.00 | 2.48 | 2.85 (0.85) | 2.27 |
| SbSeI | mp-22996 | 35470 | 1.34 | 1.66 | 2.00 | 2.49 (0.76) | 1.70 |
| SbSI | mp-23041 | 85301 | 1.62 | 1.90 | 2.27 | 2.81 (0.85) | 1.88 |
| ScN | mp-2857 | 644666 | 0.00 | 0.20 | 0.73 | 1.22 (0.33) | 0.90 |
| ScNiSb | mp-3432 | 40296 | 0.29 | 0.37 | 0.51 | 0.12 (0.04) | 0.11 |
| ScPdSb | mp-569779 | 415944 | 0.29 | 0.36 | 0.50 | 0.22 (0.06) | 0.23 |
| Si | mp-149 | 51688 | 0.58 | 0.91 | 1.59 | 1.07 (0.35) | 1.17 |
| $Si_3N_4$ | mp-988 | 170004 | 4.29 | 4.70 | 5.44 | 7.35 (1.96) | 5.10 |
| SiAs | mp-1863 | 43227 | 0.81 | 1.11 | 1.74 | 1.48 (0.45) | 1.45 |
| SiC | mp-8062 | 603798 | 1.36 | 1.55 | 2.21 | 2.61 (0.77) | 2.42 |
| SiC | mp-7140 | 86253 | 2.33 | 2.62 | 3.41 | 3.89 (1.10) | 3.33 |
| SiC | mp-11714 | 24170 | 2.23 | 2.42 | 3.05 | 3.71 (1.06) | 3.20 |
| SiC | mp-7631 | 156190 | 2.02 | 2.18 | 2.80 | 3.41 (0.98) | 2.86 |
| $SiO_2$ | mp-7000 | 154289 | 6.01 | 6.54 | 8.29 | 9.98 (2.78) | 8.90 |
| $SiP_2$ | mp-9996 | 43098 | 0.80 | 1.11 | 1.64 | 1.41 (0.45) | 1.89 |
| Sn | mp-117 | 40039 | 0.00 | 0.00 | 0.00 | 0.00 (0.00) | 0.09 |
| $Sn_2SbS_2I_3$ | mp-561134 | 23344 | 0.46 | 0.62 | 0.83 | 1.04 (0.32) | 1.50 |
| $SnBr_2$ | mp-29862 | 411177 | 2.32 | 2.65 | 3.24 | 3.82 (1.16) | 3.45 |
| $SnCl_2$ | mp-569152 | 15452 | 3.03 | 3.46 | 4.19 | 4.91 (1.43) | 3.80 |
| $SnO_2$ | mp-856 | 154960 | 1.29 | 1.71 | 2.27 | 3.41 (0.92) | 3.60 |
| SnS | mp-2231 | 52108 | 0.74 | 0.90 | 1.39 | 1.28 (0.39) | 1.23 |
| $SnS_2$ | mp-1170 | 100610 | 1.42 | 1.81 | 2.23 | 2.60 (0.82) | 2.48 |
| SnSe | mp-691 | 186650 | 0.56 | 0.80 | 1.10 | 1.23 (0.38) | 0.90 |
| $SnSe_2$ | mp-665 | 43594 | 0.69 | 1.07 | 1.46 | 1.48 (0.48) | 0.97 |
| SnTe | mp-1883 | 52489 | 0.07 | 0.36 | 0.33 | 0.51 (0.16) | 0.36 |
| $Sr_2PbO_4$ | mp-20944 | 4418 | 1.61 | 1.94 | 2.42 | 3.28 (1.03) | 1.75 |
| $Sr_2TiO_4$ | mp-5532 | 194713 | 2.09 | 2.26 | 2.51 | 4.14 (0.87) | 3.41 |
| $Sr_3Ti_2O_7$ | mp-3349 | 63704 | 1.95 | 2.13 | 2.39 | 3.96 (0.83) | 3.26 |
| $SrBiO_2Cl$ | mp-547244 | 84636 | 3.35 | 3.71 | 4.41 | 5.70 (1.59) | 3.52 |
| $SrCl_2$ | mp-23209 | 196826 | 5.34 | 6.13 | 7.82 | 9.32 (2.77) | 7.50 |
| $SrCrO_4$ | mp-542885 | 40922 | 2.98 | 3.10 | 3.27 | 4.55 (1.08) | 2.45 |
| $SrCu_2O_2$ | mp-13900 | 25002 | 1.86 | 1.89 | 2.16 | 3.45 (0.97) | 3.30 |
| $SrF_2$ | mp-981 | 40414 | 6.99 | 7.71 | 10.80 | 12.91 (3.73) | 9.60 |
| $SrGe_2$ | mp-1244 | 152799 | 0.43 | 0.57 | 0.94 | 0.99 (0.34) | 0.82 |
| $SrMoO_4$ | mp-18834 | 239418 | 4.16 | 4.29 | 4.54 | 6.65 (1.57) | 3.98 |
| SrO | mp-2472 | 163625 | 3.35 | 3.79 | 4.94 | 6.93 (1.97) | 6.10 |
| $SrPbO_3$ | mp-20489 | 78682 | 0.85 | 0.95 | 0.92 | 1.44 (0.49) | 1.78 |
| SrS | mp-1087 | 249177 | 2.48 | 3.09 | 4.34 | 4.91 (1.59) | 4.32 |
| SrSe | mp-2758 | 52429 | 2.20 | 2.74 | 3.92 | 4.40 (1.45) | 3.81 |
| $SrSeO_4$ | mp-4092 | 40923 | 4.10 | 4.64 | 5.51 | 7.25 (1.97) | 4.75 |
| $SrSnO_3$ | mp-2879 | 238971 | 2.05 | 2.36 | 2.74 | 4.17 (1.15) | 4.10 |
| $SrTaO_2N$ | mp-552454 | 411137 | 0.38 | 0.67 | 0.96 | 1.99 (0.45) | 1.99 |
| $SrTiO_3$ | mp-5229 | 94573 | 1.90 | 2.07 | 2.34 | 3.89 (0.81) | 3.25 |
| $SrZrS_3$ | mp-5193 | 154104 | 1.20 | 1.46 | 1.80 | 2.53 (0.71) | 1.00 |
| TaON | mp-4165 | 192423 | 1.71 | 1.96 | 2.25 | 3.29 (0.79) | 2.40 |
| $TeO_2$ | mp-557 | 161691 | 2.57 | 2.76 | 3.12 | 4.23 (1.13) | 3.50 |
| $TeO_2$ | mp-8377 | 90733 | 2.96 | 3.18 | 3.56 | 4.95 (1.34) | 3.41 |
| $ThO_2$ | mp-643 | 105550 | 4.39 | 4.63 | 4.97 | 7.58 (1.92) | 5.90 |
| ThOS | mp-8136 | 31654 | 0.96 | 1.33 | 1.97 | 2.33 (0.67) | 2.22 |
| ThOSe | mp-7950 | 26654 | 0.73 | 0.99 | 1.54 | 1.84 (0.53) | 1.65 |
| ThOTe | mp-3718 | 65950 | 0.15 | 0.28 | 0.81 | 0.66 (0.20) | 1.46 |
| $TiO_2$ | mp-2657 | 167953 | 2.24 | 2.40 | 2.62 | 4.27 (0.86) | 3.03 |

TABLE SI: (*Continued.*)

| Solid | MP | ICSD | PBE | EV93PW91 | AK13 | GLLB-SC | Expt. |
|---|---|---|---|---|---|---|---|
| $TiO_2$ | mp-390 | 92363 | 2.10 | 2.30 | 2.55 | 4.20 (0.87) | 3.30 |
| $Tl_2AuPS_4$ | mp-9510 | 85680 | 1.00 | 1.46 | 2.07 | 2.31 (0.74) | 2.20 |
| $Tl_2Cu_2SnS_4$ | mp-18240 | 171221 | 0.44 | 0.71 | 1.07 | 1.56 (0.47) | 1.40 |
| $Tl_2TeBr_6$ | mp-31076 | 99127 | 1.81 | 1.99 | 2.28 | 3.00 (0.90) | 2.06 |
| $Tl_2TeI_6$ | mp-31077 | 99128 | 1.57 | 1.78 | 2.02 | 2.65 (0.84) | 1.47 |
| $Tl_2TeS_3$ | mp-17172 | 391285 | 1.20 | 1.51 | 1.96 | 2.21 (0.67) | 1.60 |
| $Tl_3AsSe_3$ | mp-7684 | 15148 | 0.00 | 0.00 | 0.07 | 0.00 (0.00) | 1.30 |
| $Tl_4CdI_6$ | mp-570339 | 60756 | 2.02 | 2.51 | 3.06 | 3.33 (1.02) | 2.80 |
| TlBr | mp-22875 | 61532 | 1.92 | 2.50 | 3.58 | 3.66 (1.12) | 2.66 |
| TlCl | mp-23167 | 5253 | 2.29 | 2.89 | 4.06 | 4.32 (1.31) | 3.23 |
| $TlGaTe_2$ | mp-3785 | 16243 | 0.33 | 0.62 | 1.03 | 0.80 (0.25) | 1.20 |
| TlI | mp-23197 | 61520 | 1.63 | 2.09 | 2.96 | 3.08 (1.00) | 2.10 |
| TlI | mp-22858 | 258845 | 2.07 | 2.57 | 3.27 | 3.58 (1.12) | 2.87 |
| TlI | mp-571102 | 60491 | 2.02 | 2.57 | 3.76 | 3.51 (1.10) | 2.92 |
| $TlInSe_2$ | mp-22232 | 180272 | 0.00 | 0.15 | 0.53 | 0.17 (0.05) | 1.19 |
| $TlInTe_2$ | mp-22791 | 16245 | 0.39 | 0.68 | 1.06 | 0.94 (0.29) | 0.96 |
| TlS | mp-322 | 78161 | 0.62 | 0.95 | 1.33 | 1.33 (0.40) | 1.36 |
| $TlScS_2$ | mp-13312 | 418474 | 0.88 | 1.27 | 1.89 | 1.92 (0.56) | 1.51 |
| $TlScSe_2$ | mp-13313 | 418475 | 0.62 | 0.85 | 1.41 | 1.46 (0.43) | 0.79 |
| $TlScTe_2$ | mp-13314 | 418476 | 0.00 | 0.17 | 0.76 | 0.52 (0.14) | 0.85 |
| TlSe | mp-1836 | 104189 | 0.11 | 0.39 | 0.72 | 0.53 (0.16) | 0.73 |
| $TlTaS_3$ | mp-10795 | 412385 | 0.43 | 0.59 | 0.88 | 0.93 (0.27) | 0.78 |
| $TlTiPS_5$ | mp-558747 | 171214 | 1.06 | 1.20 | 1.46 | 1.93 (0.50) | 1.30 |
| $WS_2$ | mp-224 | 202366 | 0.98 | 1.15 | 1.41 | 1.52 (0.41) | 1.35 |
| $WSe_2$ | mp-1821 | 40752 | 0.95 | 1.12 | 1.35 | 1.50 (0.42) | 1.20 |
| Xe | mp-611517 | 43428 | 6.24 | 7.03 | 10.70 | 10.25 (3.37) | 9.29 |
| $YF_3$ | mp-2416 | 6023 | 7.89 | 8.10 | 8.66 | 13.61 (3.52) | 12.50 |
| YNiSb | mp-11520 | 105331 | 0.32 | 0.42 | 0.57 | 0.15 (0.05) | 0.18 |
| YPtSb | mp-4964 | 44970 | 0.35 | 0.67 | 0.62 | 0.27 (0.08) | 0.16 |
| $ZnAl_2S_4$ | mp-4842 | 35380 | 2.52 | 2.93 | 3.50 | 4.03 (1.20) | 3.50 |
| $ZnAs_2$ | mp-7262 | 2021 | 0.26 | 0.62 | 1.06 | 0.66 (0.20) | 0.97 |
| $ZnGa_2Se_4$ | mp-15776 | 44887 | 1.63 | 2.23 | 2.82 | 2.83 (0.83) | 2.18 |
| $ZnGa_2Te_4$ | mp-15777 | 290911 | 1.04 | 1.37 | 1.75 | 1.60 (0.50) | 1.33 |
| $ZnGeAs_2$ | mp-4008 | 68324 | 0.25 | 0.73 | 0.96 | 0.64 (0.18) | 1.15 |
| $ZnGeN_2$ | mp-2979 | 15144 | 1.75 | 2.03 | 2.41 | 3.05 (0.89) | 3.36 |
| $ZnGeP_2$ | mp-4524 | 23706 | 1.27 | 1.65 | 2.01 | 2.12 (0.64) | 2.02 |
| $ZnIn_2Te_4$ | mp-20832 | 25650 | 1.24 | 1.75 | 2.26 | 2.09 (0.62) | 1.49 |
| ZnO | mp-2133 | 162843 | 0.82 | 1.28 | 2.08 | 2.58 (0.81) | 3.44 |
| $ZnP_2$ | mp-1392 | 250015 | 0.76 | 1.08 | 1.60 | 1.44 (0.44) | 1.42 |
| ZnS | mp-10695 | 291064 | 2.12 | 2.86 | 3.71 | 3.75 (1.10) | 3.72 |
| ZnS | mp-560588 | 67453 | 2.16 | 2.88 | 3.74 | 3.79 (1.11) | 3.91 |
| ZnSb | mp-753 | 43265 | 0.13 | 0.35 | 0.60 | 0.26 (0.08) | 0.50 |
| ZnSe | mp-1190 | 77091 | 1.26 | 1.96 | 2.66 | 2.36 (0.70) | 2.82 |
| $ZnSiAs_2$ | mp-3595 | 68323 | 1.14 | 1.52 | 1.99 | 2.01 (0.63) | 1.93 |
| $ZnSiP_2$ | mp-4763 | 23680 | 1.30 | 1.72 | 2.37 | 2.26 (0.71) | 2.00 |
| $ZnSnAs_2$ | mp-5190 | 250389 | 0.08 | 0.61 | 0.93 | 0.48 (0.14) | 0.74 |
| $ZnSnO_3$ | mp-13334 | 245943 | 1.59 | 1.95 | 2.52 | 3.61 (1.05) | 3.90 |
| $ZnSnP_2$ | mp-4175 | 22179 | 0.95 | 1.48 | 1.88 | 1.86 (0.54) | 1.68 |
| $ZnSnSb_2$ | mp-4756 | 651588 | 0.02 | 0.31 | 0.48 | 0.06 (0.02) | 0.40 |
| $ZrS_2$ | mp-1186 | 604434 | 0.80 | 1.06 | 1.48 | 1.87 (0.53) | 1.68 |
| $ZrSe_2$ | mp-2076 | 109291 | 0.37 | 0.56 | 0.96 | 1.14 (0.33) | 1.18 |

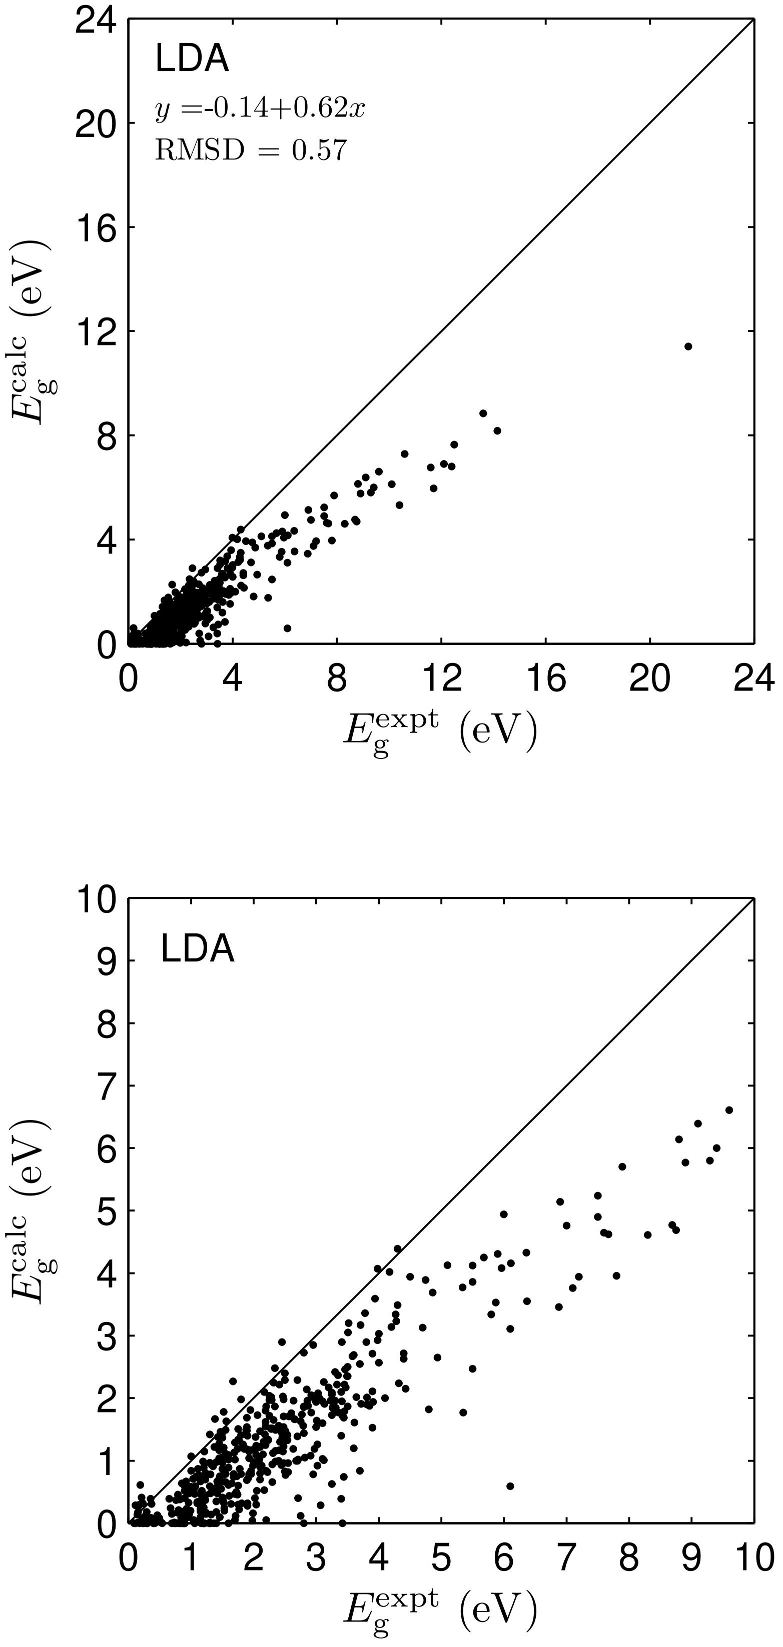


FIG. S1. Calculated versus experimental band gaps for the set of 472 solids. The lower panel is a zoom of the upper panel focusing on band gaps smaller than 10 eV. The linear regression and root-mean-square deviation of the data are also shown.

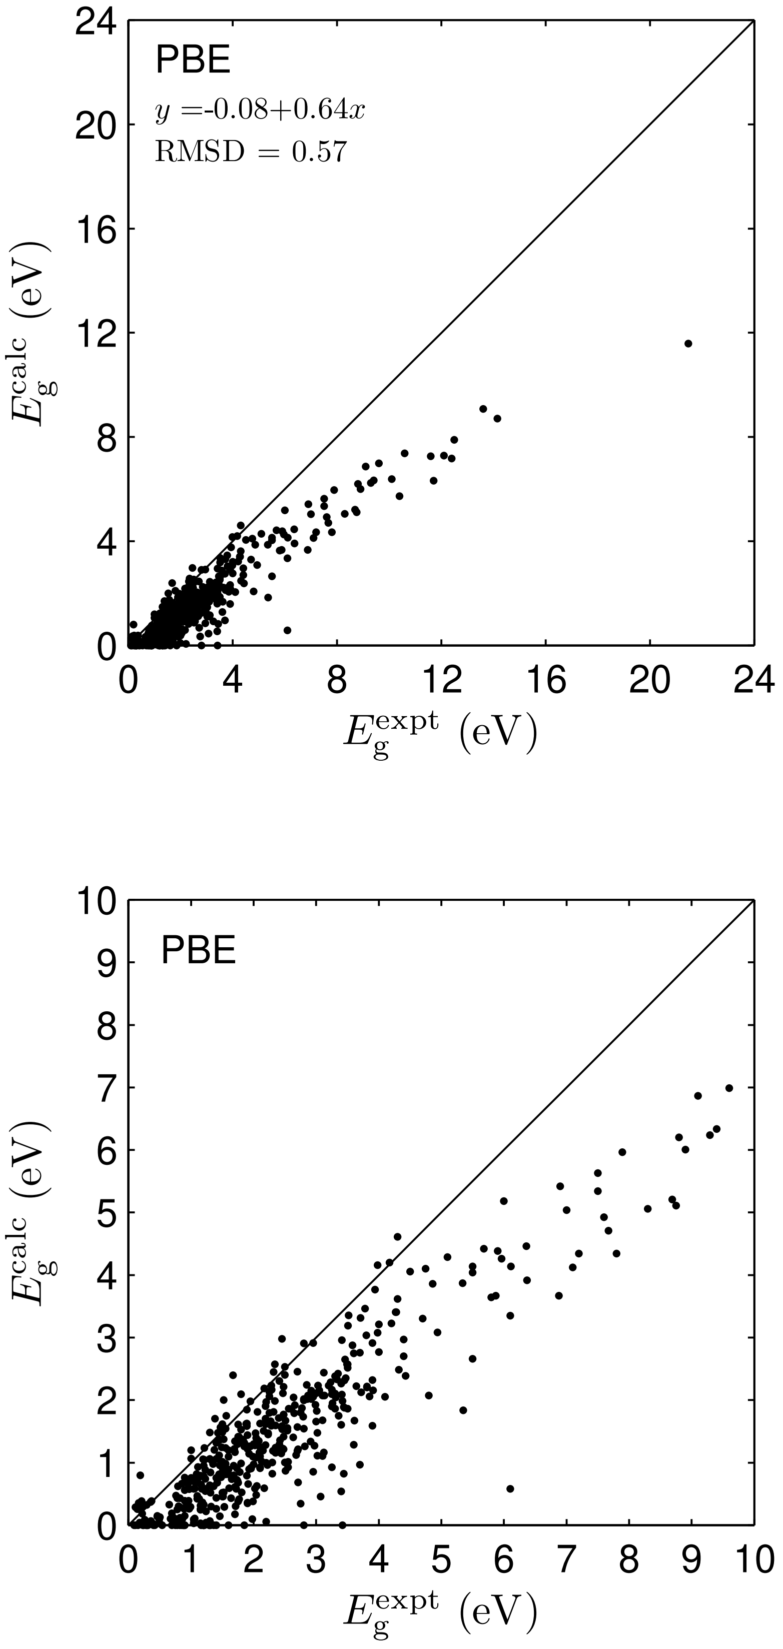


FIG. S2. Calculated versus experimental band gaps for the set of 472 solids. The lower panel is a zoom of the upper panel focusing on band gaps smaller than 10 eV. The linear regression and root-mean-square deviation of the data are also shown.

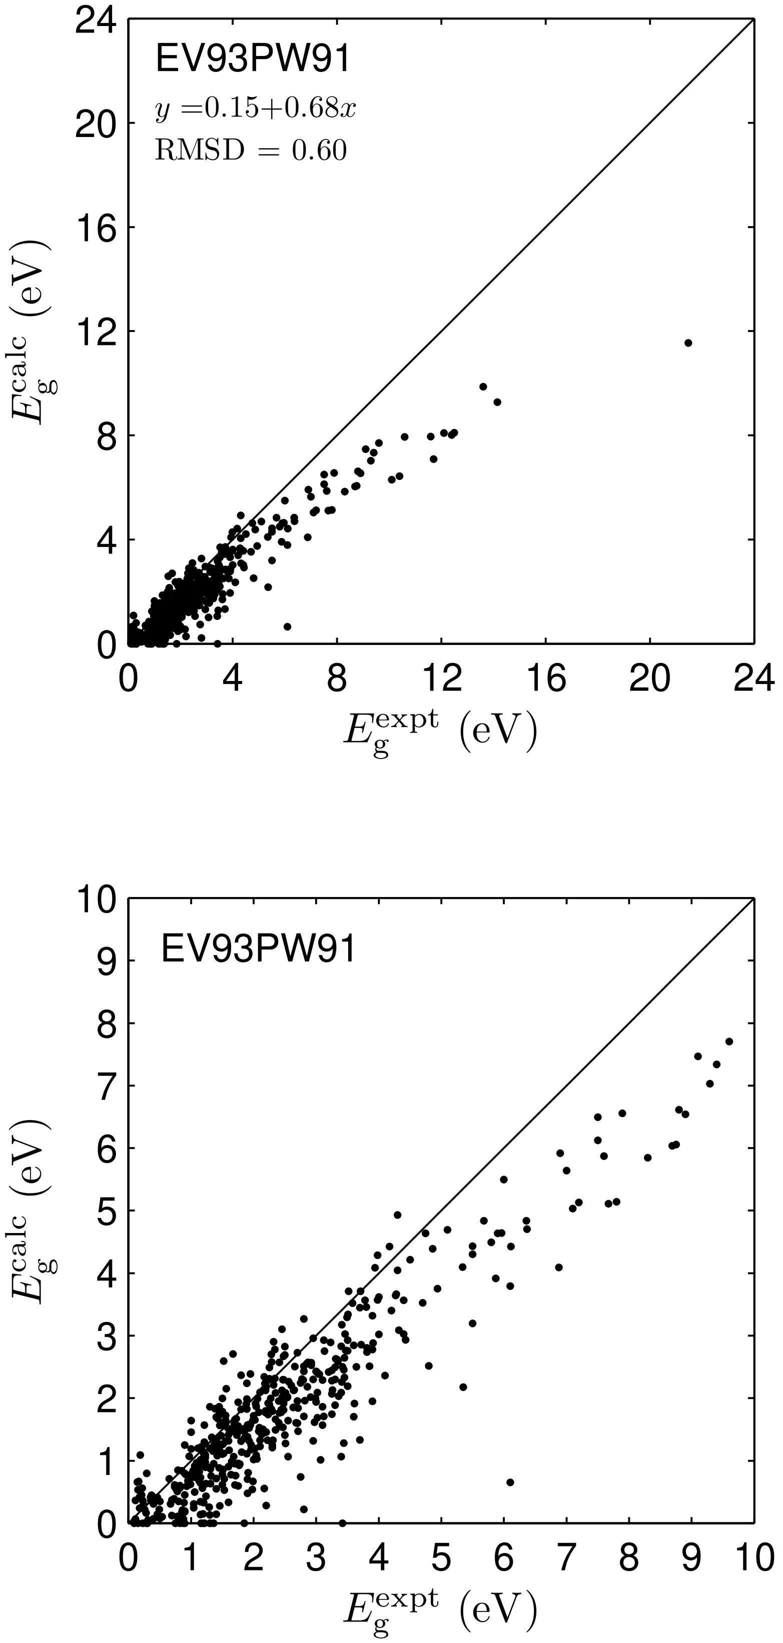


FIG. S3. Calculated versus experimental band gaps for the set of 472 solids. The lower panel is a zoom of the upper panel focusing on band gaps smaller than 10 eV. The linear regression and root-mean-square deviation of the data are also shown.

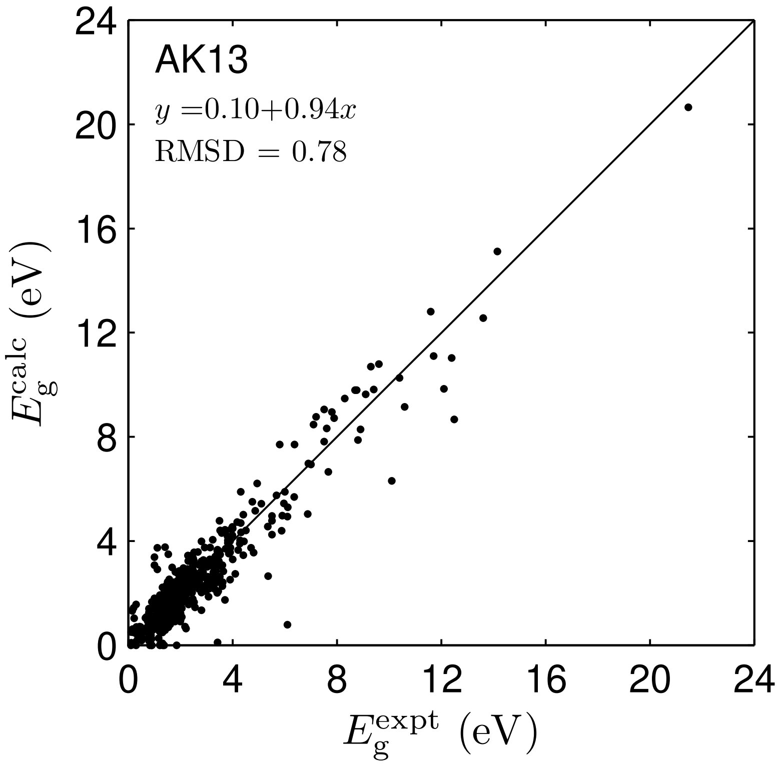


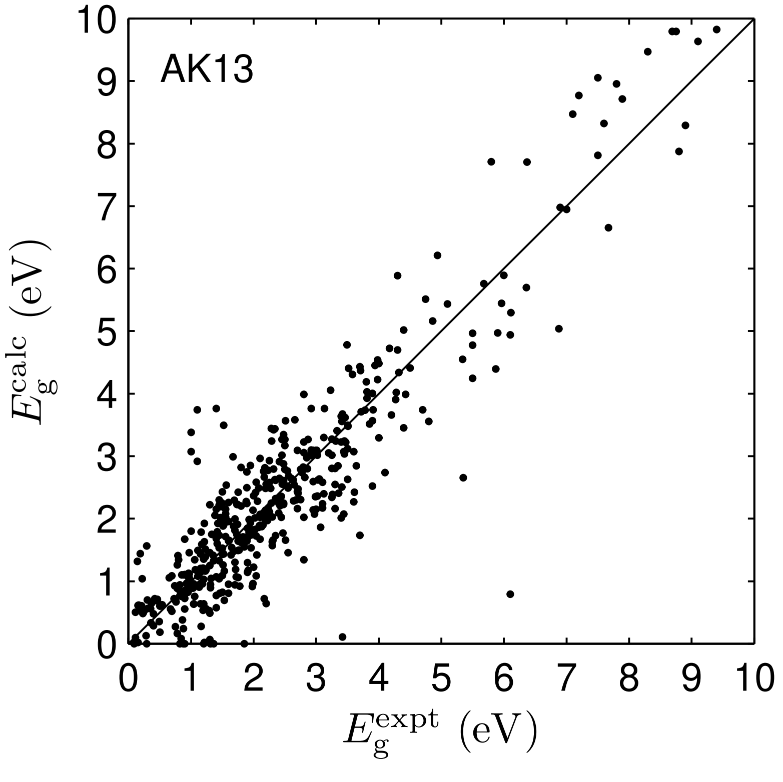


FIG. S4. Calculated versus experimental band gaps for the set of 472 solids. The lower panel is a zoom of the upper panel focusing on band gaps smaller than 10 eV. The linear regression and root-mean-square deviation of the data are also shown.

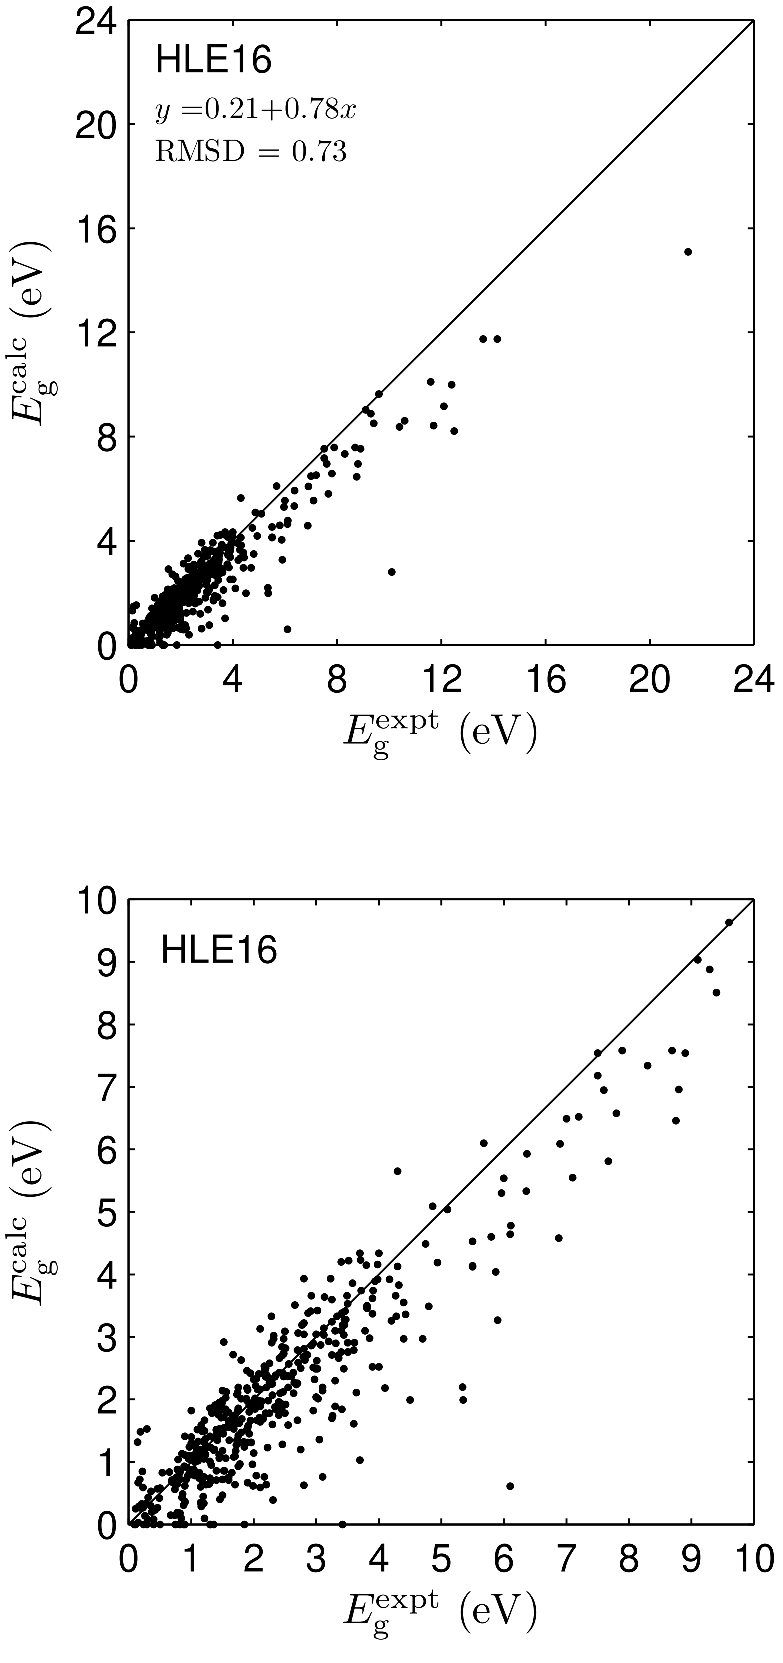


FIG. S5. Calculated versus experimental band gaps for the set of 472 solids. The lower panel is a zoom of the upper panel focusing on band gaps smaller than 10 eV. The linear regression and root-mean-square deviation of the data are also shown.

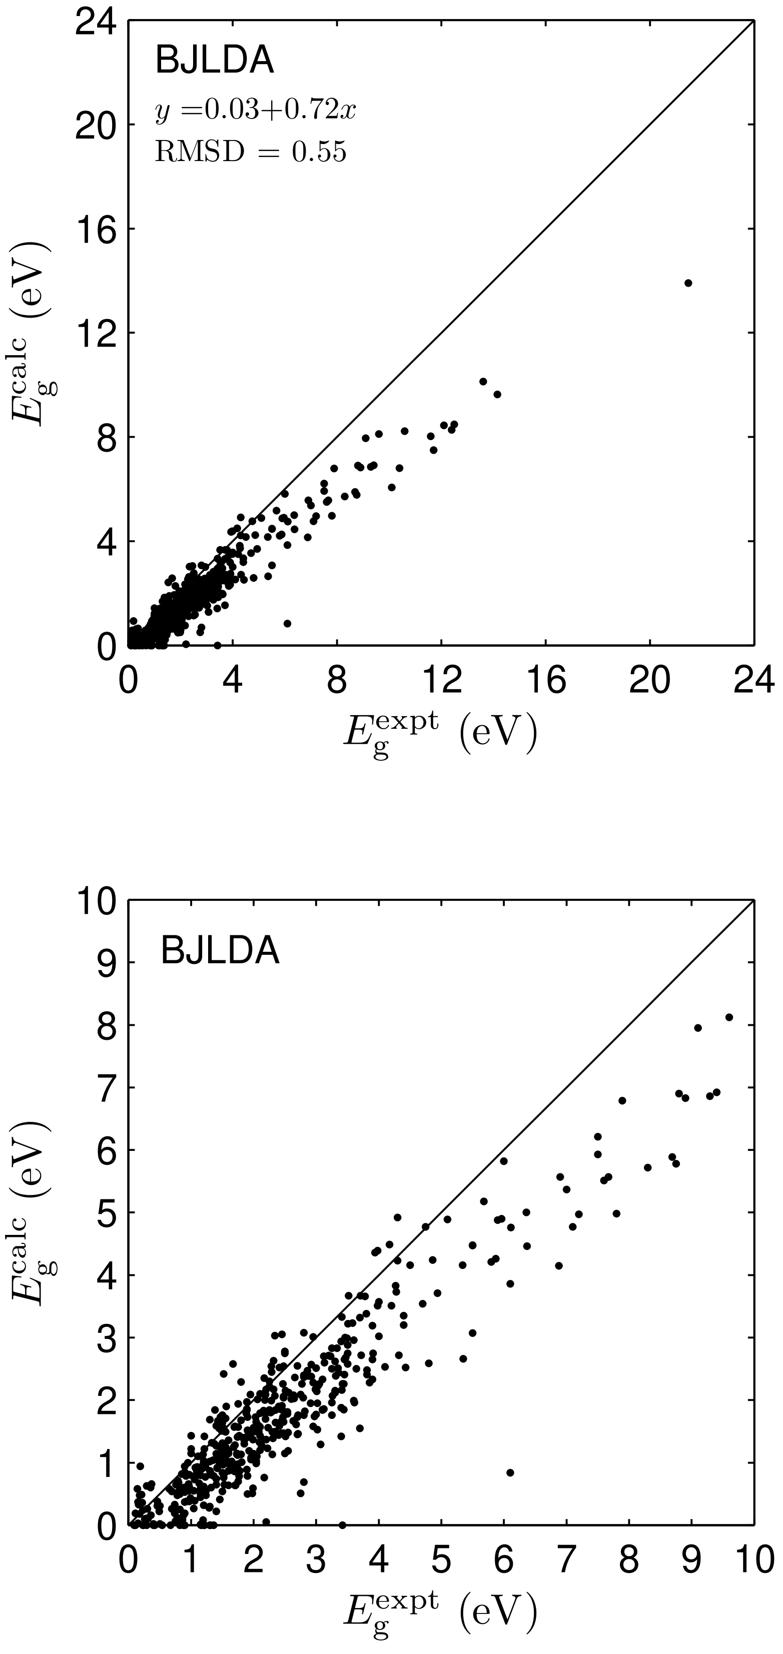


FIG. S6. Calculated versus experimental band gaps for the set of 472 solids. The lower panel is a zoom of the upper panel focusing on band gaps smaller than 10 eV. The linear regression and root-mean-square deviation of the data are also shown.

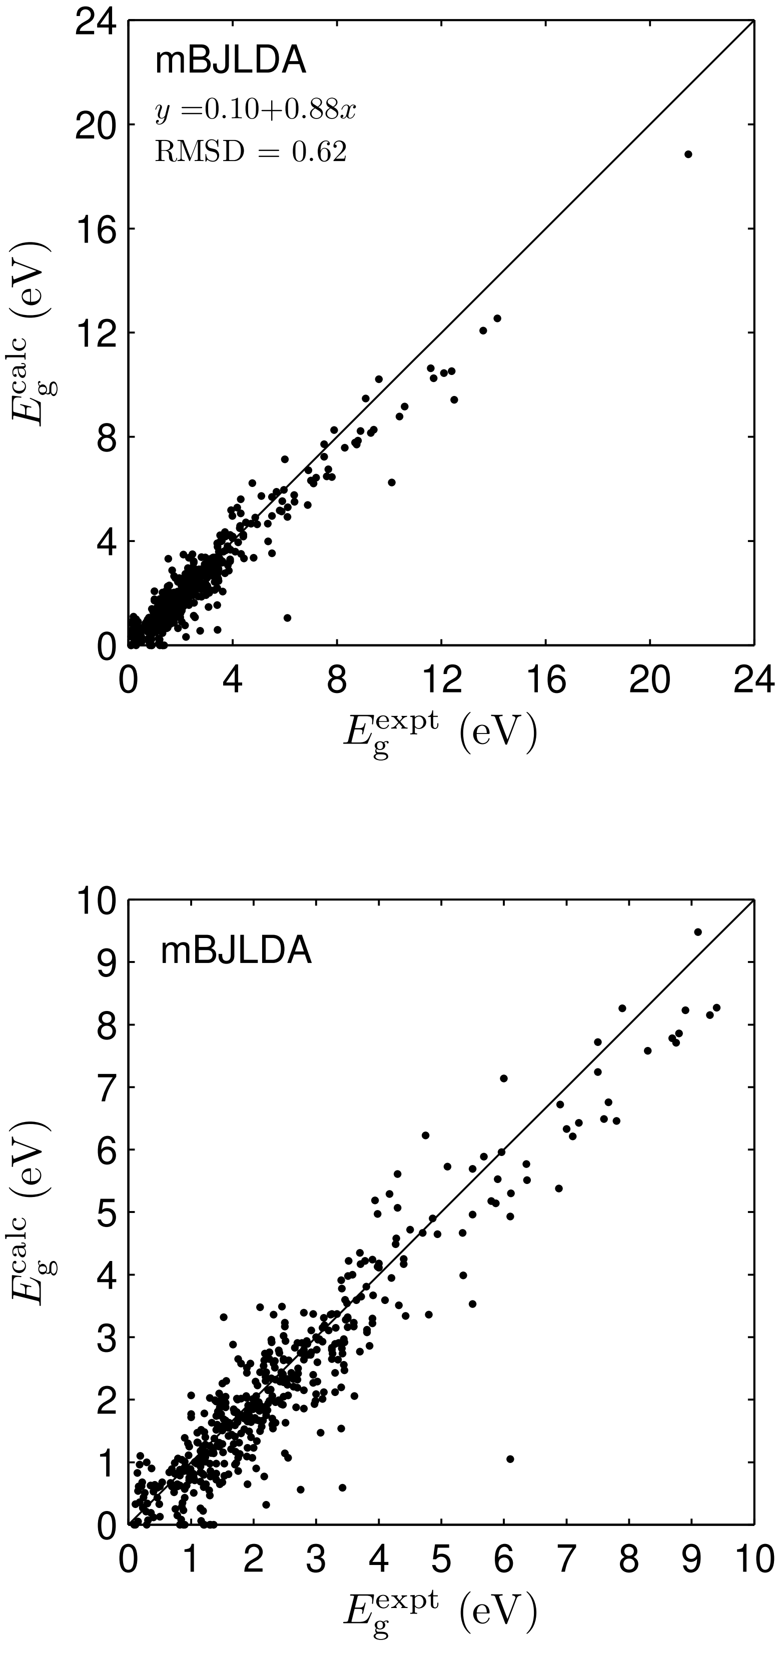


FIG. S7. Calculated versus experimental band gaps for the set of 472 solids. The lower panel is a zoom of the upper panel focusing on band gaps smaller than 10 eV. The linear regression and root-mean-square deviation of the data are also shown.

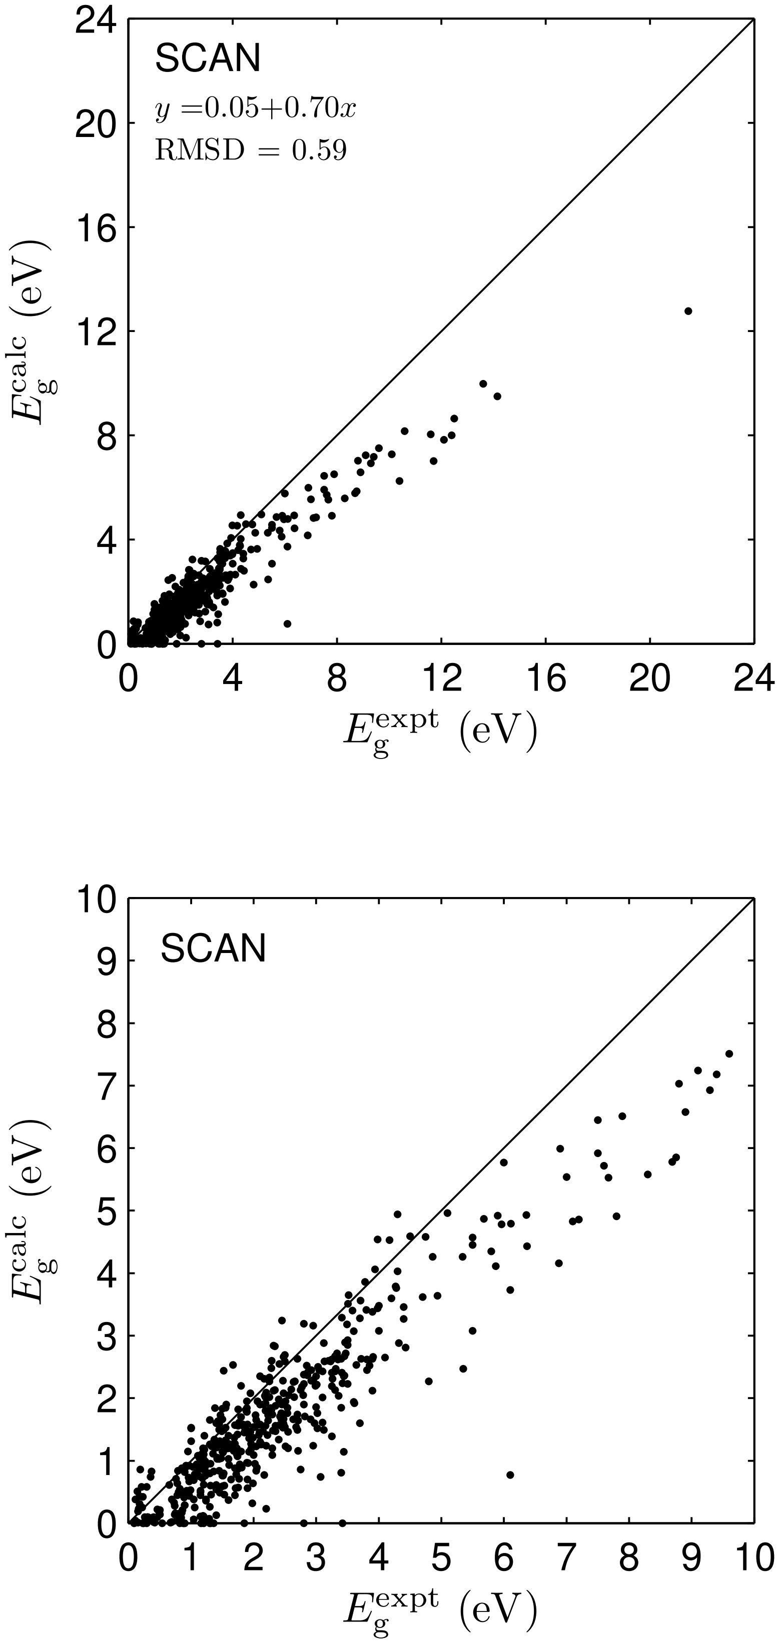


FIG. S8. Calculated versus experimental band gaps for the set of 472 solids. The lower panel is a zoom of the upper panel focusing on band gaps smaller than 10 eV. The linear regression and root-mean-square deviation of the data are also shown.

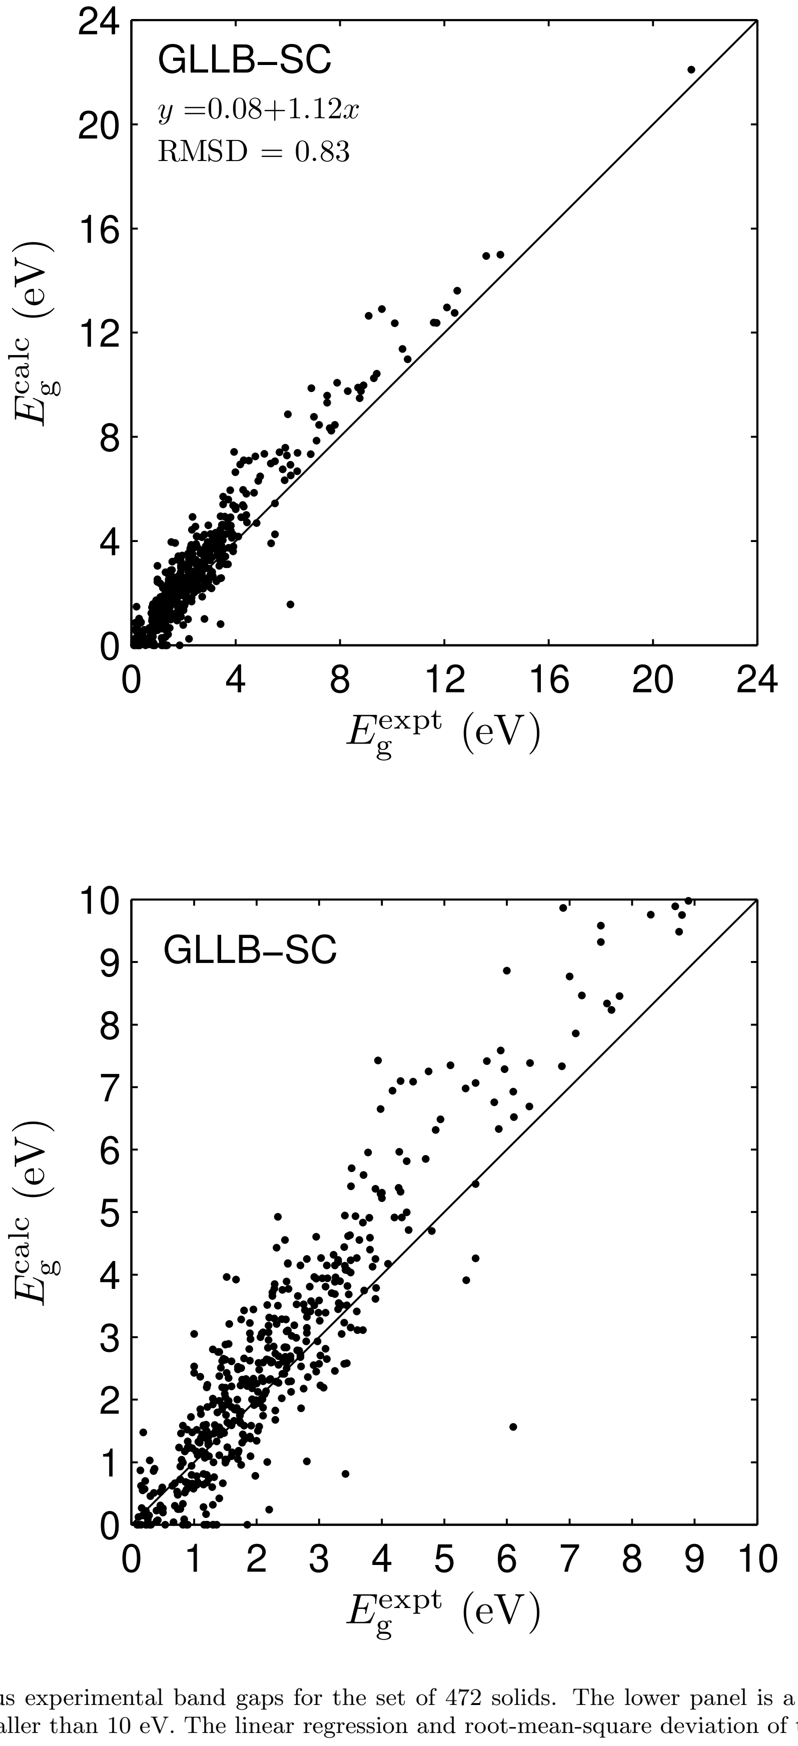


FIG. S9. Calculated versus experimental band gaps for the set of 472 solids. The lower panel is a zoom of the upper panel focusing on band gaps smaller than 10 eV. The linear regression and root-mean-square deviation of the data are also shown.

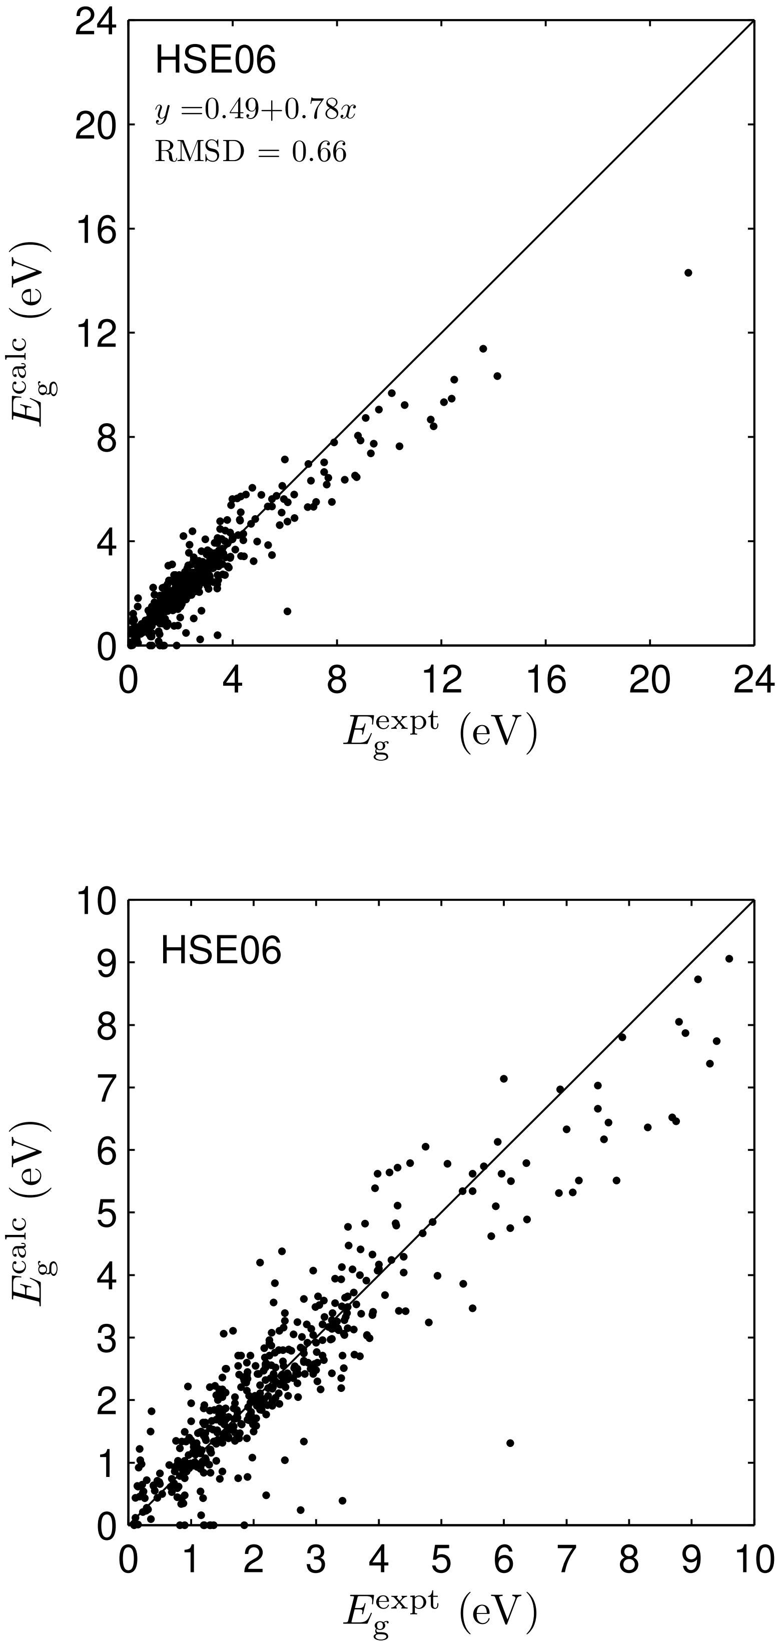


FIG. S10. Calculated versus experimental band gaps for the set of 472 solids. The lower panel is a zoom of the upper panel focusing on band gaps smaller than 10 eV. The linear regression and root-mean-square deviation of the data are also shown.

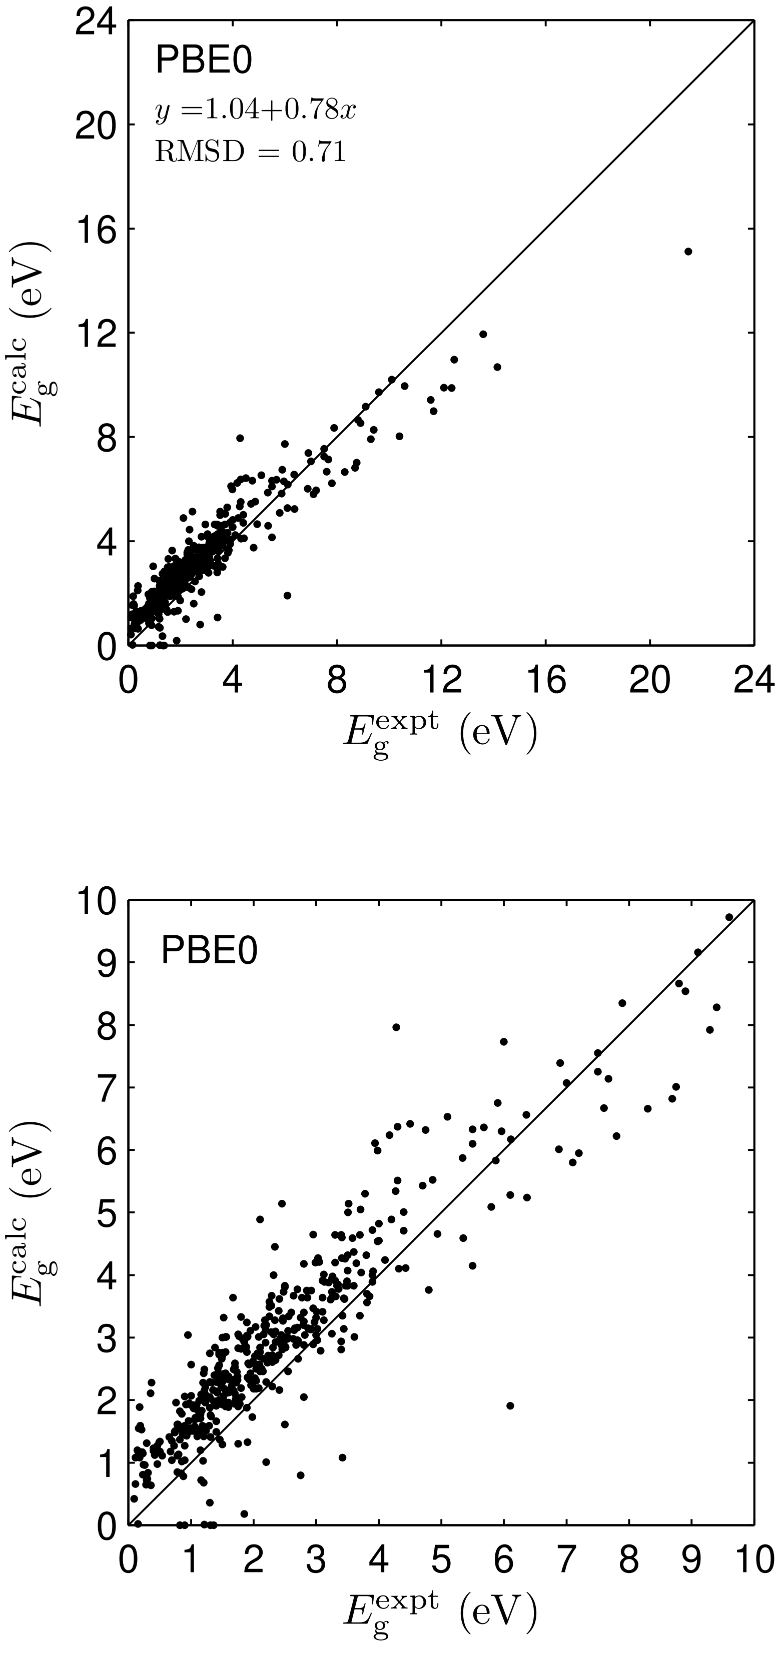


FIG. S11. Calculated versus experimental band gaps for the set of 472 solids. The lower panel is a zoom of the upper panel focusing on band gaps smaller than 10 eV. The linear regression and root-mean-square deviation of the data are also shown.

[1] A. Jain, S. P. Ong, G. Hautier, W. Chen, W. D. Richards, S. Dacek, S. Cholia, D. Gunter, D. Skinner, G. Ceder, and K. A. Persson, APL Mater. **1**, 011002 (2013).
[2] G. Bergerhoff, R. Hundt, R. Sievers, and I. D. Brown, J. Chem. Inf. Comput. Sci. **23**, 66 (1983).
[3] A. Belsky, M. Hellenbrandt, V. L. Karen, and P. Luksch, Acta Cryst. **B58**, 364 (2002).
[4] P. Borlido, T. Aull, A. W. Huran, F. Tran, M. A. L. Marques, and S. Botti, J. Chem. Theory Comput. **15**, 5069 (2019).
